# Supplementary material for: Distributional Regression Forests for Probabilistic Precipitation Forecasting in Complex Terrain
Source: arXiv:1804.02921 ancillary file (2019-02-25)
Supplement: Supplementary file 1 [file Supplement_A.pdf]

# Supplement A: Different Response Distributions

**Lisa Schlosser**
Universität Innsbruck

**Torsten Hothorn**
Universität Zürich

**Reto Stauffer**
Universität Innsbruck

**Achim Zeileis**
Universität Innsbruck

**Abstract**

In the case study presented in the main manuscript "Distributional Regression Forests for Probabilistic Precipitation Forecasting in Complex Terrain" the novel distributional regression forests are based on a Gaussian response distribution, left-censored at zero to accommodate both the non-negativity of precipitation and the point mass at zero. To assess the goodness of fit of this response distribution this supplement employs the same evaluations as in the main manuscript but based on two other distributional assumptions: A logistic distribution, left-censored at zero, is employed to potentially better capture heavy tails – and a two-part hurdle model combining a binary model for zero vs. positive precipitation and a Gaussian model, truncated at zero, for the positive precipitation observations. The latter could potentially better discriminate determinants of the occurrence of precipitation vs. the amount of precipitation given that it occurs.

*Keywords*: random forests, GAMLSS, hurdle model, logistic, Gaussian.

## 1. Introduction

This supplement extends the case study presented in Section 3.4 of the main manuscript by carrying out the same evaluation at 15 stations using two alternative response distributions for the power-transformed daily precipitation sums.

To assess how appropriate the distributional assumption (left-censored Gaussian distribution with censoring point zero; or zero-censored for short) is, two questions are considered: (1) Are the tails of the distribution captured appropriately by a Gaussian distribution or are *heavier tails* required? (2) Is the point mass at zero (= no rain) driven by the same determinants as the positive observations (= rain) or should this be captured by a *separate parameter*? For (1) we compare the zero-censored Gaussian with a *zero-censored logistic* distribution and for (2) a Gaussian *hurdle model* (or two-part model with binary and zero-truncated parts) is employed instead of the zero-censored Gaussian.

Just as in the main manuscript the performance of the distributional forest is also compared with other commonly-used distributional regression models using the same data set. The models are learned on data from the first 24 years (1985–2008) and evaluated on the following 4 years (2009–2012). Table 2 of the manuscript provides an overview of all models considered and their specifications. As a reminder the approaches are briefly summarized below.

- *Distributional forest:* All predictor variables are considered for learning a forest where subsampling is employed for each tree. Parameters are estimated by adaptive local likelihood based on forest weights.

- *EMOS* (Gneiting *et al.* 2005): Ensemble model output statistics uses the ensemble mean of total precipitation as regressor in the location submodel and the corresponding ensemble standard deviation in the scale submodel. The parameters are estimated by maximum likelihood.
- *Prespecified GAMLSS:* Smooth additive splines are selected for the most relevant predictors based on meteorological expert knowledge following Stauffer *et al.* (2017). The model is estimated by maximum penalized likelihood using a backfitting algorithm (Stasinopoulos and Rigby 2007).
- *Boosted GAMLSS:* Smooth additive splines are selected automatically from all available variables, using non-cyclic boosting for parameter estimation (Hofner *et al.* 2016; Messner *et al.* 2017). The optimal stopping point for the iterations is determined based on a (computationally intensive) out-of-bag bootstrap estimate of the log-likelihood.

## 2. Alternative response distributions

The main manuscript employs a Gaussian distribution with probability density function $f$ (PDF) and cumulative distribution function $F$ (CDF) given by

$$f_{\text{Gaussian}}(Y;\mu,\sigma) = \frac{1}{\sigma}\cdot\phi\left(\frac{Y-\mu}{\sigma}\right) \tag{1}$$

$$F_{\text{Gaussian}}(Y;\mu,\sigma) = \Phi\left(\frac{Y-\mu}{\sigma}\right) \tag{2}$$

where $\phi$ and $\Phi$ are the PDF and the CDF of the standard normal distribution $\mathcal{N}(0,1)$.

An alternative distribution with several similar properties but with heavier tails is the logistic distribution. The PDF and CDF are given by

$$f_{\text{logistic}}(Y;\mu,\sigma) = \frac{\exp\left(-\frac{Y-\mu}{\sigma}\right)}{\sigma\cdot\left(1+\exp\left(-\frac{Y-\mu}{\sigma}\right)\right)^2} \tag{3}$$

$$F_{\text{logistic}}(Y;\mu,\sigma) = \frac{1}{1+\exp\left(-\frac{Y-\mu}{\sigma}\right)}. \tag{4}$$

Both distributions have to be adapted in our case study to accommodate that precipitation is non-negative with a point mass at zero (= no rain). Two common strategies for this are to employ either *left-censoring at zero* or a *hurdle* (or two-part) approach, combining a binary (zero vs. greater) and a truncated (positive) part (see Long 1997 or Winkelmann and Boes 2009 for an overview of both techniques).

- *Censored distribution:* For a chosen distribution with PDF $f$ and CDF $F$ the log-likelihood function of the corresponding zero-censored distribution is

$$\ell_{\text{cens}}(\mu,\sigma;Y) = \begin{cases} \log\left\{f(Y;\mu,\sigma)\right\}, & \text{if } Y>0 \\ \log\left\{F(0;\mu,\sigma)\right\}, & \text{if } Y=0 \end{cases} \tag{5}$$

as stated in Equation 2.1.1 of the main manuscript for the Gaussian special case. For positive values of $Y$ the censored version of the PDF equals the original non-censored version. For $Y = 0$ the censored density function takes the values of the probability mass lying left of the censoring point. Therefore, the parameters $\mu$ and $\sigma$ control both aspects, the point mass and the positive part of the distribution.

- *Hurdle model (or two-part model, Cragg 1971; Mullahy 1986):* An additional parameter $\nu$ describing the probability that there is any precipitation at all, i.e., $\nu = \mathbb{P}(Y > 0)$, is included in the model. The three-parameter log-likelihood function for the full hurdle model with parameter vector $\boldsymbol{\theta} = (\mu, \sigma, \nu)$ is

$$\ell_{\text{hurdle}}(\mu, \sigma, \nu; Y) = \begin{cases} \log\left\{\nu \cdot \frac{f(Y;\mu,\sigma)}{1-F(0;\mu,\sigma)}\right\}, & \text{if } Y > 0 \\ \log(1-\nu), & \text{if } Y = 0. \end{cases} \tag{6}$$

  For $Y = 0$ the probability for no rain is $1 - \nu$. For $Y > 0$ the probability $\nu$ for no rain is multiplied with the PDF, left-truncated at zero. In contrast to the censored model, there is thus a dedicated parameter $\nu$ controlling the point mass while the other parameters $\mu$ and $\sigma$ only influence the distribution of the positive observations.

Note that, due to the logs in the first part of Equation 6, the log-likelihood of the hurdle model can be separated additively into a part that depends only on $\nu$ (for all observations) and a part that depends on $\mu$ and $\sigma$ (for only the positive observations). Therefore, in a GAMLSS approach, the log-likelihood of the $\nu$ submodel can be maximized separately from the log-likelihood of the $\mu$ and $\sigma$ submodels to maximize the overall log-likelihood. Hence in all GAMLSS models considered subsequently a binary logit model is employed for $Y = 0$ vs. $Y > 0$ and a zero-truncated Gaussian model in the case of $Y > 0$. Similarly, for the distributional forest two separate forests are employed with a binary and a zero-truncated Gaussian response, respectively. For comparison with the zero-censored distributions the combined three-parameter hurdle model as formulated in Equation 6 is employed.

All models are evaluated using the continuous ranked probability score (CRPS). For the censored models the closed form formulas provided by Jordan *et al.* (2018) are used while a numerical approximation is employed for the hurdle models.

## 3. Stations

Out of the 95 observation stations 15 are considered for this supplemental study (see Figure 1). They have been selected to cover a wide range regarding geographical location, altitude, and which of the competing models performed best in the single-split setting reported in Section 3.4 of the main manuscript.

Selected stations: Axams, Lech, Zuers, See im Paznaun, Jungholz, Ladis-Neuegg, Oetz, Ochsengarten-Obergut, Ginzling, Rotholz, Walchsee, Koessen, Innervillgraten, Matrei in Osttirol, St. Johann im Walde. See also Supplement B ("Stationwise Evaluation") for more details.

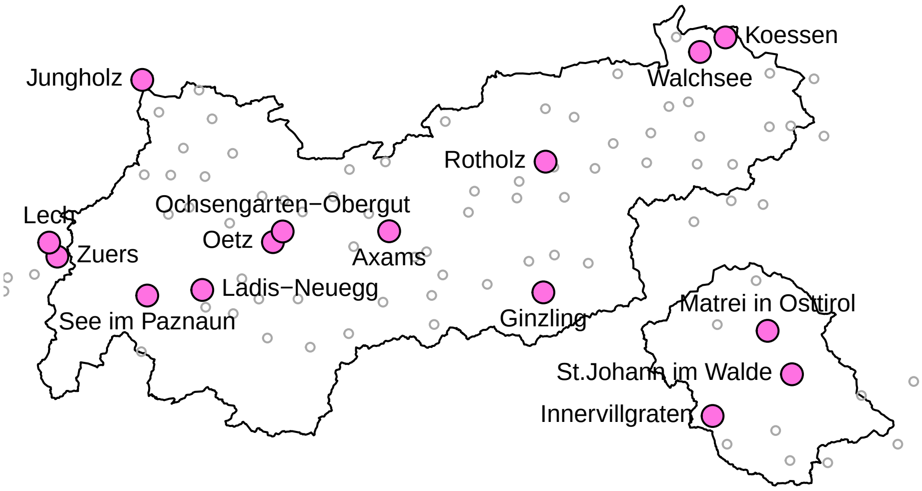


Figure 1: Map of Tyrol with all 95 observation stations and the 15 considered stations highlighted in pink.

## 4. Results

*CRPS for all distributions by model and station*

Each panel of Figure 2 compares the CRPS across the three distributions considered: *cgaussian* (zero-censored Gaussian), *hgaussian* (Gaussian hurdle model), and *clogistic* (zero-censored logistic). The four different models considered are coded by both colors and symbols and connected by lines for easier comparison between models. As the average CRPS (i.e., the difficulty of the prediction problem) varies substantially by station, separate panels are employed for each station.

- For the distributional forest all three distributions perform very similarly for all stations. Thus, it appears to be very robust against missspecifications of the distribution.
- Also for the prespecified GAMLSS all three distributions lead to almost the same results and no clear advantage of one or the other distribution can be detected.
- Similarly, for the EMOS model and the boosted GAMLSS all distributions lead to comparable CRPS for all stations. However, there is some more variation in CRPS across distributions compared to the distributional forest.

*Note:* When applying the hurdle model at stations Oetz and Innvervillgraten the prespecified GAMLSS could not be estimated (using the R package **gamlss**) due to numerical issues in the fitting algorithm. Therefore, this method is not represented in the two corresponding panels of Figure 2.

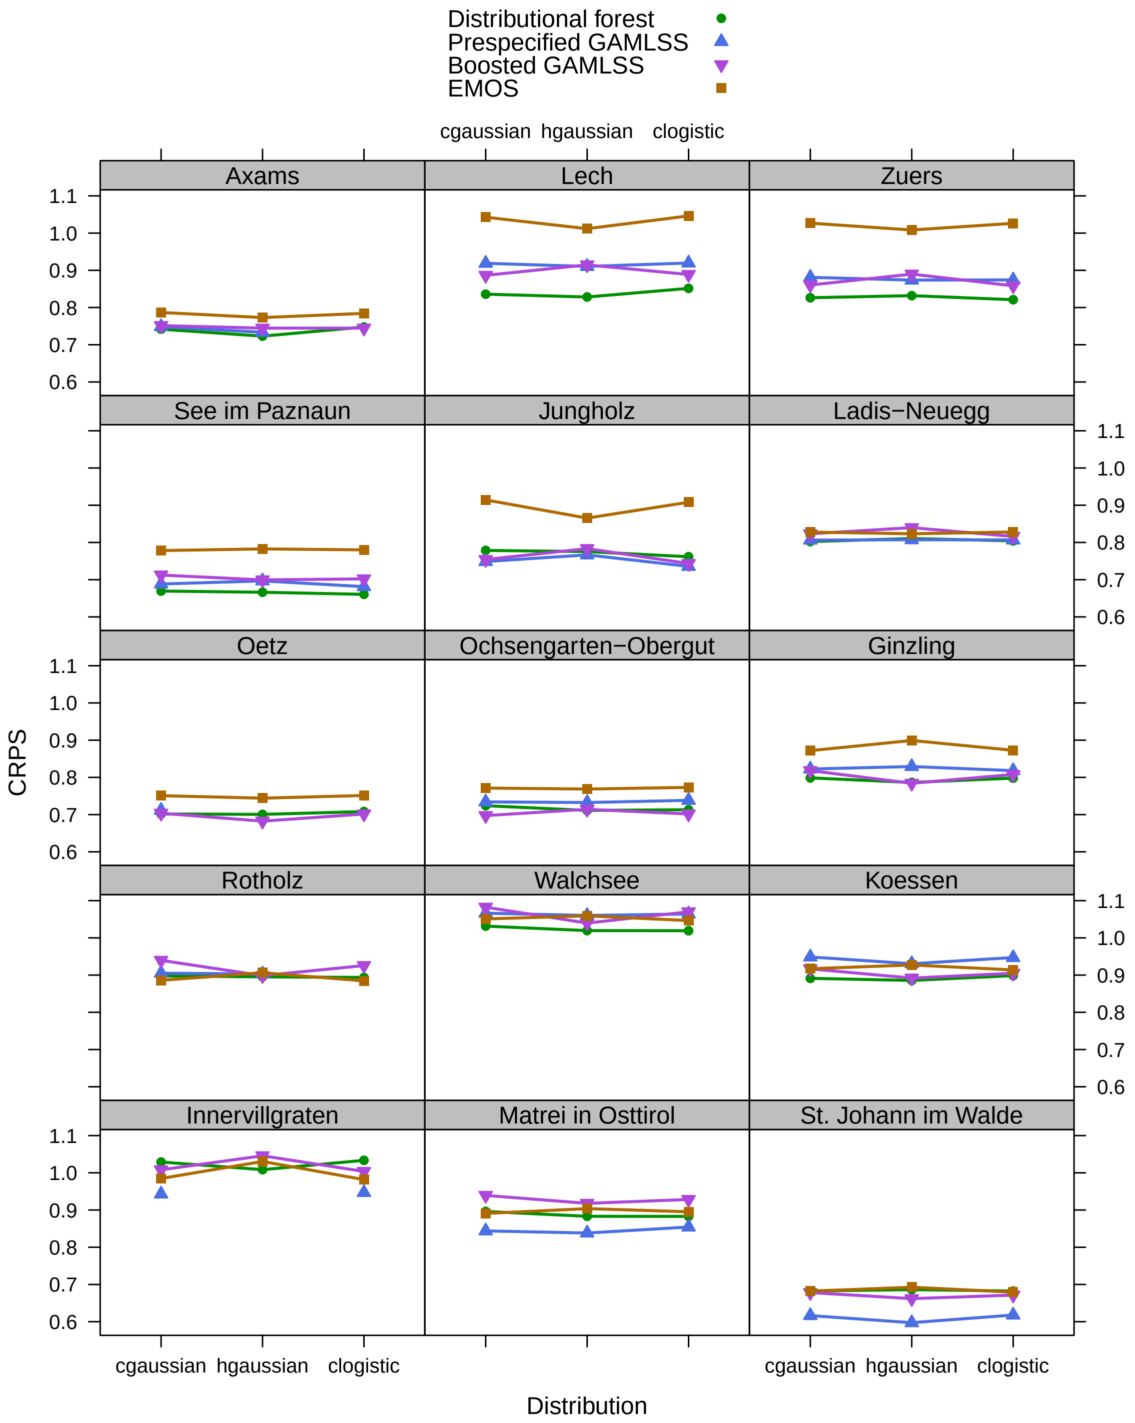


Figure 2: CRPS values (lower = better) across the three distributions for all four models and 15 stations.

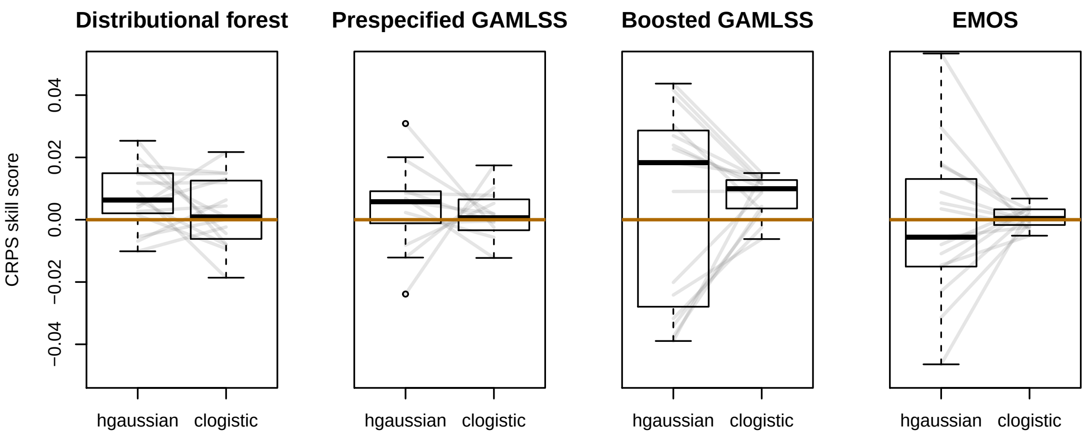


Figure 3: CRPS skill score (higher = better) for hurdle Gaussian and censored logistic distributions in reference to the censored Gaussian distribution (orange horizontal line). Gray lines correspond to the 15 stations that are aggregated in the boxplot.

### *CRPS skill score in reference to zero-censored Gaussian*

To aggregate the CRPS results across stations, CRPS skill scores are visualized with boxplots in Figure 3, using the zero-censored Gaussian distribution as the reference distribution (orange horizontal line at zero). The underlying skill scores for each station are also included in the graphic by gray lines.

- As before, there are only slight variations for the distributional forest, mostly between ±1%. While the median CRPS skill score over the 15 stations for the Gaussian hurdle model is slightly better than for the simpler zero-censored Gaussian model, this advantage is very small and not systematic across stations.
- Again, for the prespecified GAMLSS the results are very similar as for the distributional forest showing only a slight advantage of the Gaussian hurdle model, however, not for all stations.
- For the boosted GAMLSS, the Gaussian hurdle is quite close to the zero-censored Gaussian reference but shows a high variation, while the zero-censored logistic performs slightly better.
- For EMOS, the median skill score for both Gaussian hurdle and zero-censored logistic are very close to the zero-censored Gaussian reference. However, as for the boosted GAMLSS the variation for the hurdle model is much higher than for the censored model.

Altogether it can be stated that for this application the zero-censored Gaussian distribution seems to be an appropriate choice while the other two distributions are also reasonable alternatives. However, they do not lead to a pronounced overall improvement in performance for this application.

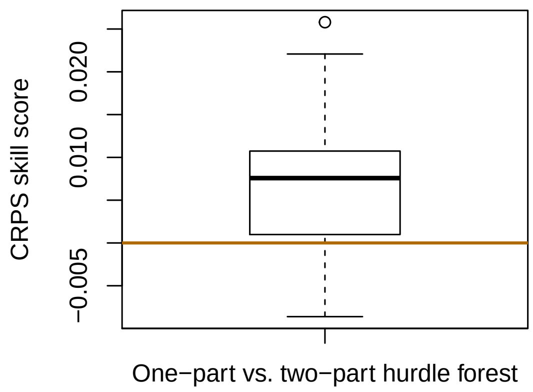


Figure 4: CRPS skill score (higher = better) for the one-part hurdle distributional forest in reference to the two part hurdle distributional forest (orange horizontal line).

## 5. Discussion

This supplement shows that the zero-censored Gaussian models from the main manuscript and the alternative distributional specifications in this supplement perform at least similarly. For some combinations of models and stations, the Gaussian hurdle leads to small improvements on average but typically with more variability (especially for EMOS and the boosted GAMLSS). Furthermore, for the boosted GAMLSS the zero-censored logistic distribution shows slightly better results, however, only within a range of less than 2% and not for all stations. Therefore, the main manuscript focuses on the zero-censored Gaussian model which is well-established in the probabilistic precipitation forecasting literature. Moreover, the distributional forest can be shown to be rather robust against distributional (mis-)specifications compared to the other models.

As a final consideration, we briefly remark that the distributional forest also allows for a different hurdle model specification. Previously, we argued that for GAMLSS/EMOS the log-likelihood of the hurdle model can be separated additively and hence the maximum likelihood fit can be obtained by fitting two separate models for $\nu$ on one hand and $\mu$ and $\sigma$ on the other. And therefore the same two-part approach was also adopted for the distributional forests. However, an additional alternative is to fit a single distributional forest based on the three-parameter log-likelihood from Equation 6. When all three parameters change simultaneously across the covariates, then this specification can be expected to perform somewhat better. Whereas when different variables/effects drive the different model parameters, then the two-part approach implemented in this supplement should perform somewhat better. In this particular case study, though, neither approach performs clearly better as Figure 4 reveals. The figure depicts CRPS skill scores for the 15 stations of the one-part hurdle models with the two-part hurdle model as the reference. Clearly, both hurdle specifications perform very similarly with skill scores being mostly below 1%.

# References

Cragg JG (1971). "Some Statistical Models for Limited Dependent Variables with Application to the Demand for Durable Goods." *Econometrica*, **39**(5), 829–844.

Gneiting T, Raftery AE, Westveld III AH, Goldman T (2005). "Calibrated Probabilistic Forecasting Using Ensemble Model Output Statistics and Minimum CRPS Estimation." *Monthly Weather Review*, **133**(5), 1098–1118. doi:10.1175/mwr2904.1.

Hofner B, Mayr A, Schmid M (2016). "**gamboostLSS**: An R Package for Model Building and Variable Selection in the GAMLSS Framework." *Journal of Statistical Software*, **74**(1), 1–31. doi:10.18637/jss.v074.i01.

Jordan A, Krueger F, Lerch S (2018). "Evaluating Probabilistic Forecasts with **scoringRules**." *Journal of Statistical Software*. Forthcoming.

Long JS (1997). *Regression Models for Categorical and Limited Dependent Variables*. Sage Publications, Thousand Oaks.

Messner JW, Mayr GJ, Zeileis A (2017). "Non-Homogeneous Boosting for Predictor Selection in Ensemble Post-Processing." *Monthly Weather Review*, **145**(1), 137–147. doi:10.1175/mwr-d-16-0088.1.

Mullahy J (1986). "Specification and Testing of Some Modified Count Data Models." *Journal of Econometrics*, **33**(3), 341–365. doi:10.1016/0304-4076(86)90002-3.

Stasinopoulos DM, Rigby RA (2007). "Generalized Additive Models for Location Scale and Shape (GAMLSS) in R." *Journal of Statistical Software*, **23**(7), 1–46. doi:10.18637/jss.v023.i07.

Stauffer R, Umlauf N, Messner JW, Mayr GJ, Zeileis A (2017). "Ensemble Post-Processing of Daily Precipitation Sums over Complex Terrain Using Censored High-Resolution Standardized Anomalies." *Monthly Weather Review*, **45**(3), 955–969. doi:10.1175/mwr-d-16-0260.1.

Winkelmann R, Boes S (2009). *Analysis of Microdata*. 2nd edition. Springer-Verlag, New York.

**Affiliation:**

Lisa Schlosser, Reto Stauffer, Achim Zeileis
Universität Innsbruck
Department of Statistics
Faculty of Economics and Statistics
Universitätsstr. 15
6020 Innsbruck, Austria
E-mail: Lisa.Schlosser@uibk.ac.at, Reto.Stauffer@uibk.ac.at,
Achim.Zeileis@R-project.org
URL: https://www.uibk.ac.at/statistics/personal/schlosser-lisa/,
https://retostauffer.org/,
https://eeecon.uibk.ac.at/~zeileis/

Torsten Hothorn
Universität Zürich
Institut für Epidemiologie, Biostatistik und Prävention
Hirschengraben 84
CH-8001 Zürich, Switzerland
E-mail: Torsten.Hothorn@R-project.org
URL: http://user.math.uzh.ch/hothorn/
