# Supplementary material for: Distributional Regression Forests for Probabilistic Precipitation Forecasting in Complex Terrain
Source: arXiv:1804.02921 ancillary file (2019-02-25)
Supplement: Supplementary file 2 [file Supplement_B.pdf]

# Supplement B: Stationwise Evaluation

**Lisa Schlosser**
Universität Innsbruck

**Torsten Hothorn**
Universität Zürich

**Reto Stauffer**
Universität Innsbruck

**Achim Zeileis**
Universität Innsbruck

**Abstract**

In the case study presented in the main manuscript "Distributional Regression Forests for Probabilistic Precipitation Forecasting in Complex Terrain" the novel distributional regression forests are evaluated and compared with other distributional regression approaches on 95 meteorological stations. Moreover, further details – including a cross-validation analysis – are performed for only one station, Axams. To show that Axams is a fairly typical station and similar insights can be obtained for other stations as well, this supplement presents the same analysis as in Section 3.3 of the main manuscript for 14 further meteorological stations.

*Keywords*: random forests, GAMLSS, evaluation, meteorological stations.

# 1. Setup

## 1.1. Models

As introduced in Section 3.2 of the main manuscript, a distributional forest based on a Gaussian distribution, left-censored at zero, is evaluated together with three other zero-censored Gaussian models. Table 2 of the manuscript provides an overview of all models considered and their specifications. As a reminder the approaches are briefly summarized below.

- *Distributional forest:* All predictor variables are considered for learning a forest where subsampling is employed for each tree. Parameters are estimated by adaptive local likelihood based on forest weights.

- *EMOS* (Gneiting *et al.* 2005): Ensemble model output statistics uses the ensemble mean of total precipitation as regressor in the location submodel and the corresponding ensemble standard deviation in the scale submodel. The parameters are estimated by maximum likelihood.

- *Prespecified GAMLSS:* Smooth additive splines are selected for the most relevant predictors based on meteorological expert knowledge following Stauffer *et al.* (2017). The model is estimated by maximum penalized likelihood using a backfitting algorithm (Stasinopoulos and Rigby 2007).

- *Boosted GAMLSS:* Smooth additive splines are selected automatically from all available variables, using non-cyclic boosting for parameter estimation (Hofner *et al.* 2016;

Messner *et al.* 2017). The optimal stopping point for the iterations is determined based on a (computationally intensive) out-of-bag bootstrap estimate of the log-likelihood.

### 1.2. Learning and test samples

The models are always learned on data from 24 years and tested on the remaining 4 years. Splitting the data into these two subsets is done in two different ways leading to the two following evaluation settings.

- *Single split*: The data is time-ordered. The learning data consists of the first 24 years (1985–2008) and the testing data of the following 4 years (2009–2012).
- *Cross-validation*: In order to not just split the data at one splitpoint the 28 years are randomly split into 7 blocks of 4 years which are not necessarily successive. Each of the blocks is chosen once as testing data while the remaining 6 blocks are the learning data. This procedure is repeated 10 times resulting in a 10 times 7-fold cross-validation framework.

The performances of the models are compared based on numerical and graphical evaluations.

### 1.3. Numerical evaluation

Several numerical summary statistics are computed in both settings. For the single-split setting one value is calculated for each observation in the test data and then their mean is reported. For the cross-validation setting, the same is done for all 70 splits considered and again their mean is reported. The following summary statistics are used.

- *CRPS*: The continuous ranked probability score (CRPS) is calculated to assess the predictive performance in terms of full probabilistic forecasts.
- *Computation time*: For all models fitting times and predictions times are measured on the same 16-core Linux computer. In particular, *fit time* refers to the time needed to fit the model to the learning data in a particular split. The *predict time* refers to the time needed to compute the out-of-sample prediction. In the single-split setting, the predictions are computed observation by observation, i.e., emulating the realistic setup where predictions are made once the new NWP model outputs become available. In the cross-validation setting, the predictions for the full 4-year out-of-sample period in one go. Although this is not realistic in this particular application, it might be an interesting quantity for comparing the competing regression approaches.

*Note:* For a few splits in the cross-validation, the prespecified GAMLSS (as computed by the `R` package **gamlss**) failed, leading to `NA`s in the corresponding summary statistics. As mentioned by Hofner *et al.* (2016) such problems are not unusual because GAMLSS “can be unstable, especially when it comes to selecting possibly different sets of variables for multiple distribution parameters”.

### 1.4. Graphical evaluation

The following methods of visualization are applied to provide further means of comparison of all models but also to investigate on the distributional forest in particular.

- *Boxplot of the CRPS skill score:* With EMOS as the reference model the CRPS skill scores are calculated on each of the 70 splits considered in the cross-validation setting and illustrated in a boxplot.

- *Barplot of variable importance:* For the distributional forest it is investigated which variables have the strongest influence on the model and its goodness of fit. For each variable this is measured based on mean decrease in CRPS after permutation. The 10 variables showing the highest values in the single-split setting are listed in a barplot.

- *Residual QQ plots:* For each of the models an out-of-sample residual QQ plot for the single-split setting provides a graphical goodness-of-fit assessment.

- *PIT histograms:* Similarly, the out-of-sample probability integral transform (PIT) in the single-split setting is employed as an alternative goodness-of-fit visualization.

The Residual QQ plots and the PIT histograms visualize the same values, however, on different scales. For each observation $y$ of the test sample the corresponding PIT value is calculated by applying the probability function $F(y; \hat{\mu}, \hat{\sigma})$ with the estimated distribution parameters plugged in. The resulting values can either be plotted in a histogram (PIT histogram) or be plotted against the corresponding quantiles of a standard normal distribution (residual QQ plot) for a continuous variable $Y$. To account for the point mass at 0, for each observation equal to 0 the corresponding PIT value is multiplied with a randomized value following a uniform distribution on $[0, 1]$. In that way these values are apportioned on those bins of the histogram that would not contain any values because no observation is beneath 0.

# 2. Stations

Out of the 95 observation stations 15 are considered for this supplemental study. They have been selected to cover a wide range regarding geographical location, altitude, and which of the competing models performed best in the single-split setting reported in Section 3.4 of the main manuscript.

Selected stations: Axams, Lech, Zuers, See im Paznaun, Jungholz, Ladis-Neuegg, Oetz, Ochsengarten-Obergut, Ginzling, Rotholz, Walchsee, Koessen, Innervillgraten, Matrei in Osttirol, St. Johann im Walde.

# 3. Results

## 3.1. Forecasting skill

Based on the out-of-sample CRPS results it can be concluded that the distributional forest generally performs well on all stations and is typically close to (e.g., Lech) or somewhat better than the (next-)best method (e.g., See im Paznaun and Ginzling). Naturally, there is more variation in the single-split results with another model performing better than the distributional forest. However, in the cross-validation such differences often even out, showing that distributional forests are on par. Examples for this include Rotholz, Matrei in Osttirol,

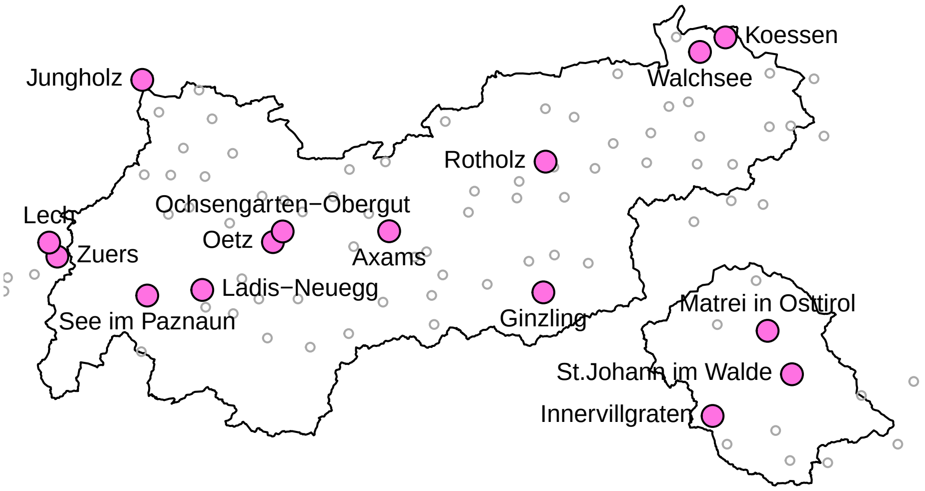


Figure 1: Map of Tyrol with all 95 observation stations and the 15 considered stations highlighted in pink.

and Ochsengarten-Obergut, where the best models in the single split are EMOS, prespecified GAMLSS and boosted GAMLSS, respectively. The only station, where another model performs clearly better than distributional forests in both settings, is St. Johann im Walde.

Overall, the results support the conclusion that distributional forests perform well for this prediction task – they are often on par and sometimes even better than the other models considered. Moreover, it is shown that the results for Axams are fairly typical and not particularly unusual compared to the other stations considered.

### 3.2. Computation time

Distributional forests are comparable with respect to the computation times to the other two flexible GAMLSS models. Only the basic EMOS model is clearly the fastest. Moreover, unlike the other models, the boosted GAMLSS requires a time-consuming cross-validation to determine the optimal stopping value `mstop`. This is crucial for selecting the appropriate model complexity and relevant covariates and hence cannot be neglected in the analysis.

The observation-wise prediction times in the single-split setting are in the same order of magnitude for the three flexible distributional models. However, when many predictions are computed simultaneously in the cross-validation setting, then distributional forests are slower than the GAMLSS models. The reason for this is that the GAMLSS can set up the model matrices once and then carry out a matrix product while the distributional forest necessitates fitting a separate set of parameters for each observation-specific weight vector.

### 3.3. Variable importance

Two NWP model outputs based on total precipitation (`tp_max` and `tp_mean`) are clearly the most important predictors for precipitation at all stations considered. The remaining variables typically follow with some margin and vary slightly in their exact order. However, they typically encompass some NWP model outputs for total precipitation, total column-integrated condensate, and temperature differences.

### 3.4. Calibration

The PIT histograms and residual QQ plots show that overall all four models are reasonably well-calibrated at the majority of stations while at some stations they all fit better (e.g., at station Oetz) or worse (e.g., at station Matrei in Osttirol) than on average. For several stations, however, the boosted GAMLSS does not capture the heavy upper tail as well as the other methods which is best seen in the residual QQ plots but also the PIT histograms.

# Axams

Longitude: 11.276
Latitude: 47.231
Altitude: 890.000

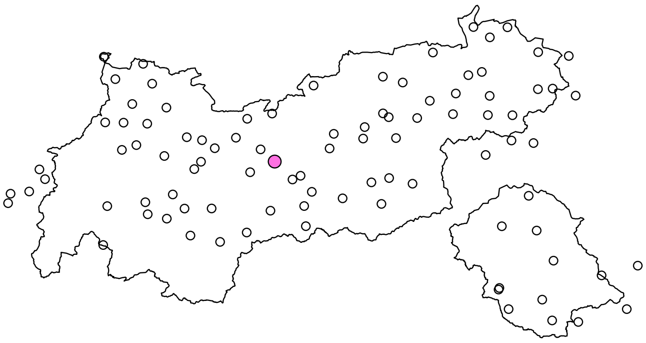

## Overview

| Model | Single split CRPS | Fit time | Predict time | 10 times 7-fold cross-validation CRPS | Fit time | Predict time |
|---|---|---|---|---|---|---|
| Distributional forest | 0.742 | 74.418 | 0.317 | 0.665 | 82.432 | 4.462 |
| Prespecified GAMLSS | 0.748 | 58.052 | 0.265 | 0.678 | 92.379 | 0.406 |
| Boosted GAMLSS | 0.750 | 119.222 | 0.107 | 0.678 | 137.179 | 0.146 |
| *(mstop selection)* | | 1534.557 | | | 2349.737 | |
| EMOS | 0.787 | 0.094 | 0.006 | 0.706 | 0.100 | 0.006 |

## CRPS skill score (cross-validation, reference: EMOS)

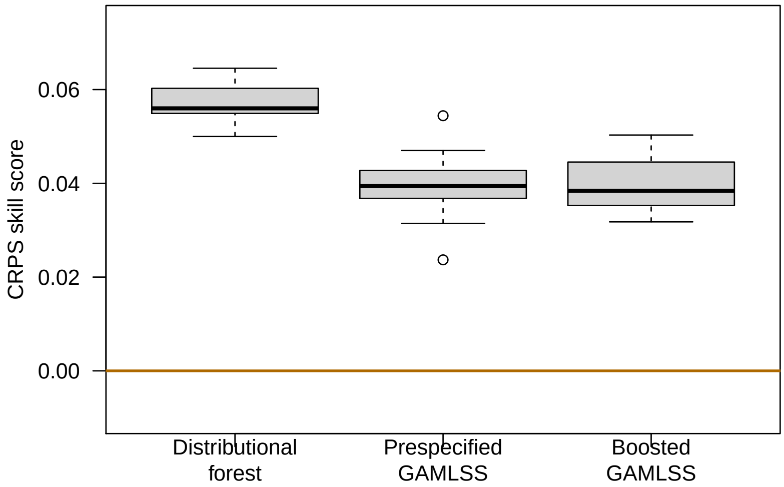


## Variable importance

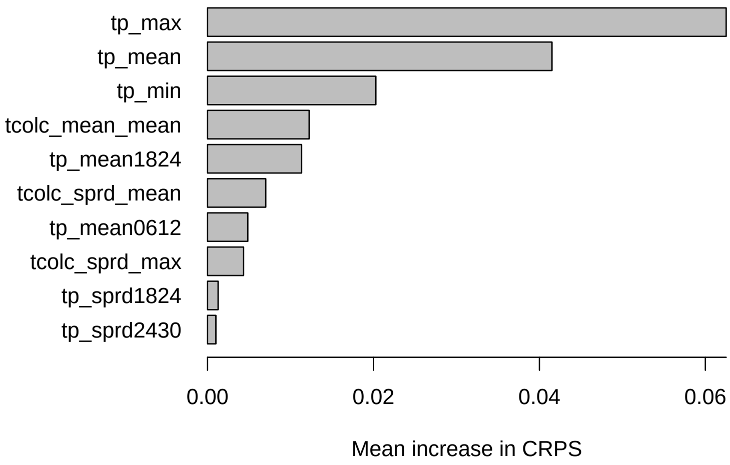

## Residual QQ plots

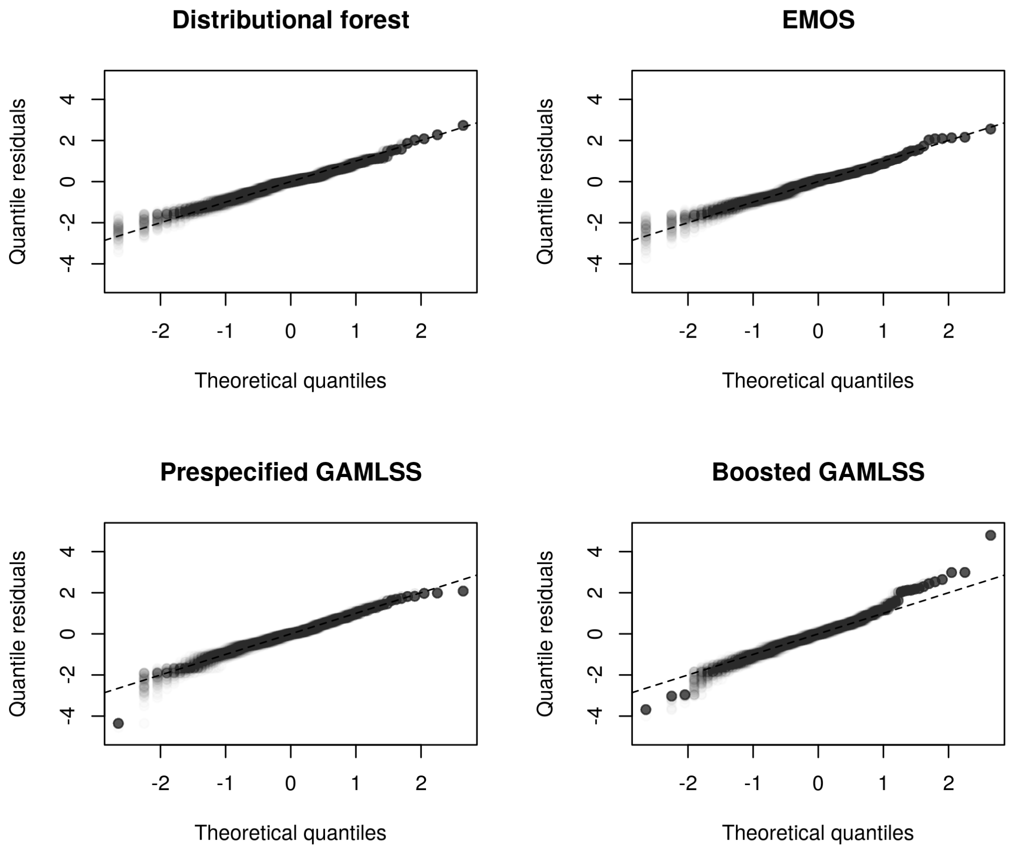


## PIT histograms

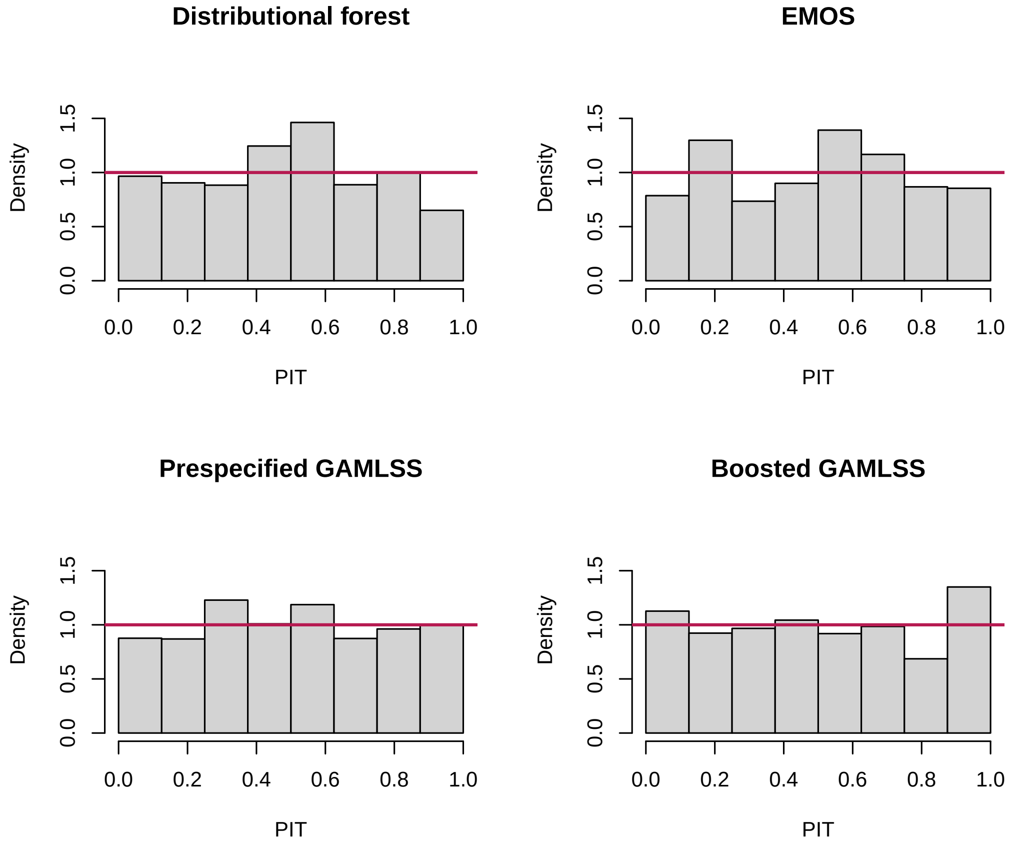

# Lech

Longitude: 10.136
Latitude: 47.205
Altitude: 1480.000

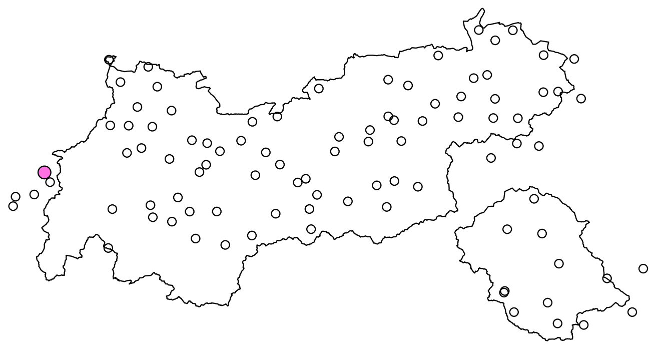

### Overview

| Model | Single split CRPS | Fit time | Predict time | 10 times 7-fold cross-validation CRPS | Fit time | Predict time |
|---|---|---|---|---|---|---|
| Distributional forest | 0.836 | 70.374 | 0.315 | 0.844 | 78.994 | 4.241 |
| Prespecified GAMLSS | 0.919 | 65.873 | 0.264 | 0.870 | 101.552 | 0.378 |
| Boosted GAMLSS | 0.886 | 110.290 | 0.102 | 0.846 | 128.370 | 0.132 |
| *(mstop selection)* | | 1414.442 | | | 2343.186 | |
| EMOS | 1.043 | 0.082 | 0.006 | 1.013 | 0.090 | 0.005 |

### CRPS skill score (cross-validation, reference: EMOS)

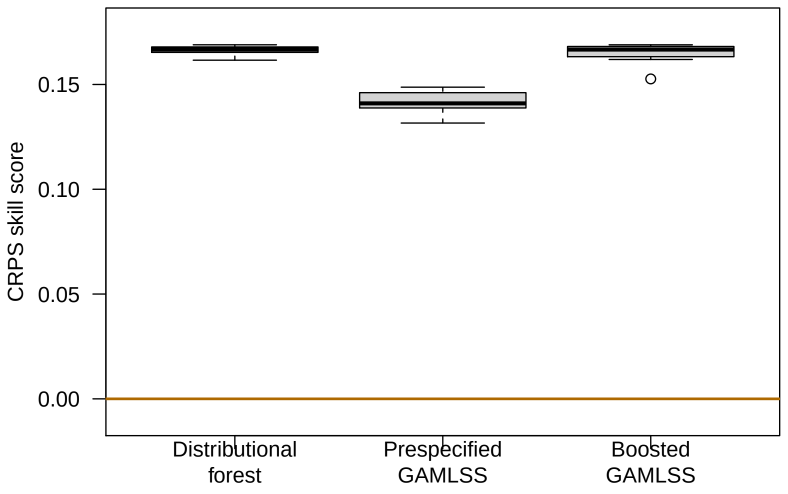


### Variable importance

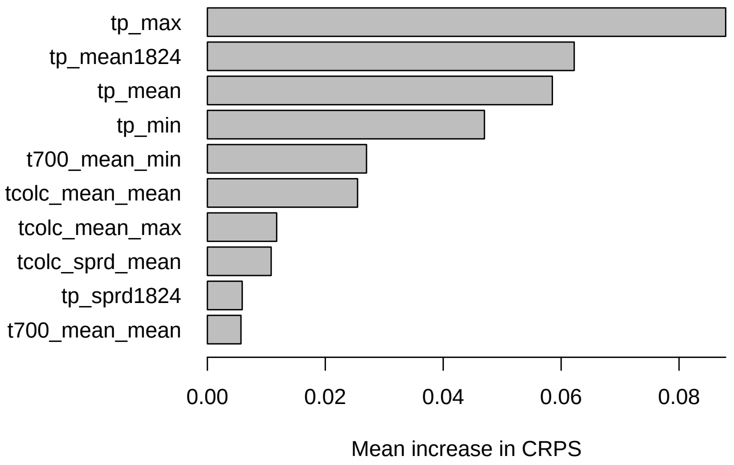

## Residual QQ plots

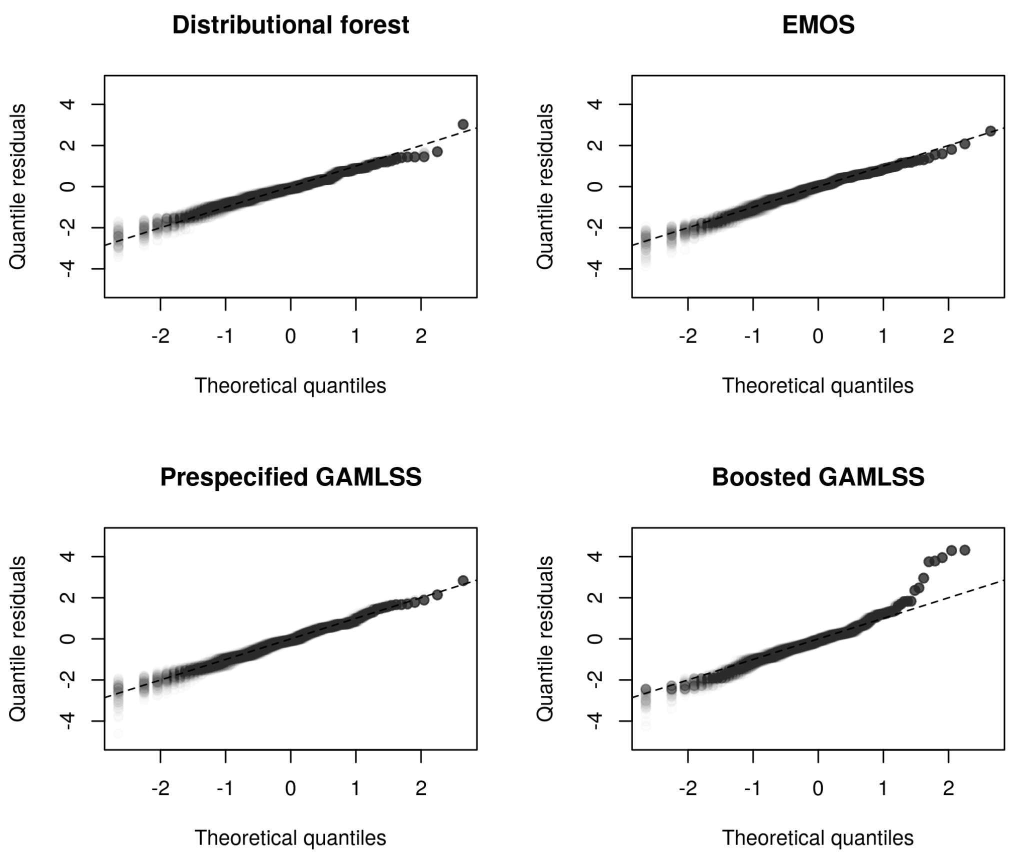


## PIT histograms

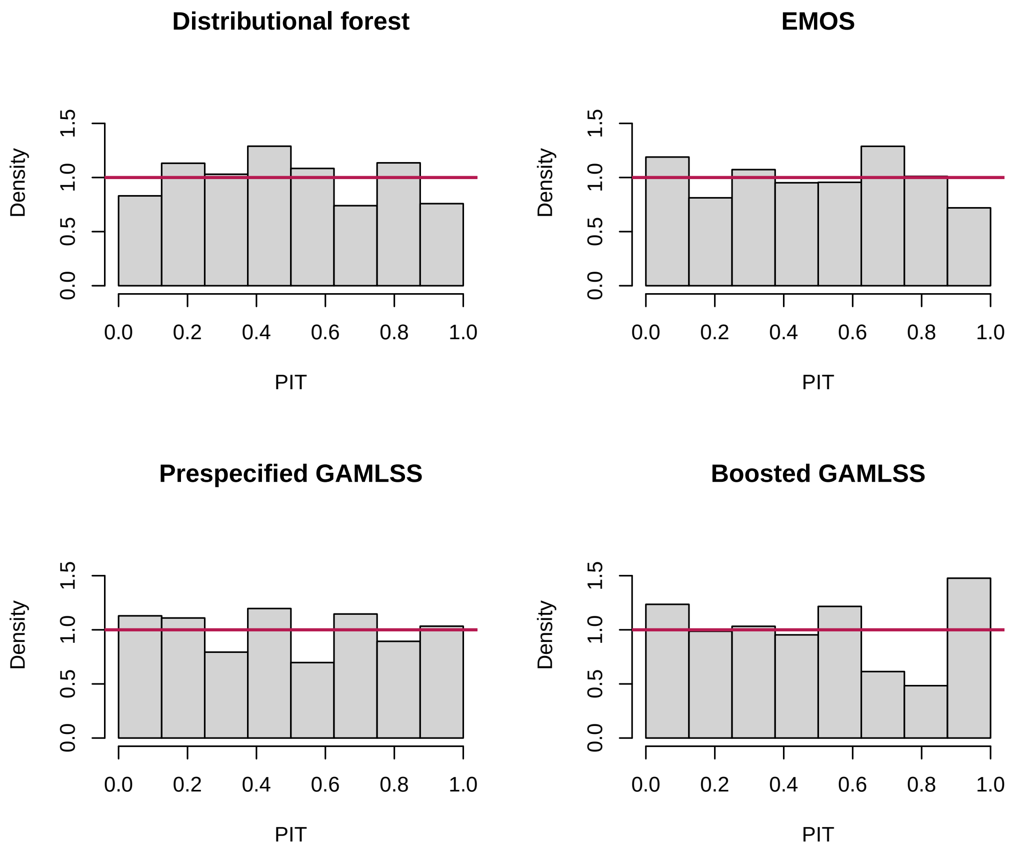

# Zuers

Longitude: 10.163
Latitude: 47.173
Altitude: 1707.000

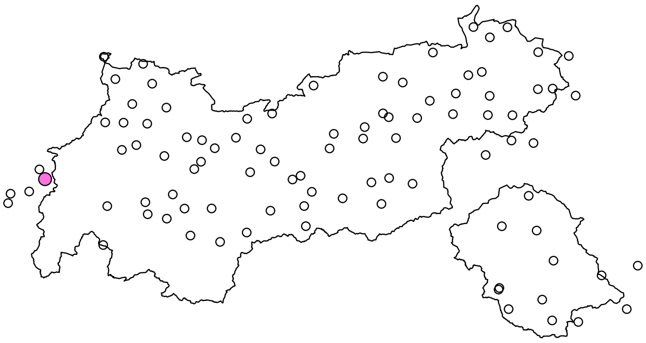

## Overview

| Model | Single split CRPS | Fit time | Predict time | 10 times 7-fold cross-validation CRPS | Fit time | Predict time |
|---|---|---|---|---|---|---|
| Distributional forest | 0.826 | 68.961 | 0.308 | 0.831 | 79.290 | 4.351 |
| Prespecified GAMLSS | 0.881 | 75.015 | 0.263 | 0.874 | 136.526 | 0.387 |
| Boosted GAMLSS | 0.861 | 110.309 | 0.104 | 0.830 | 131.773 | 0.140 |
| *(mstop selection)* | | 1409.283 | | | 2350.917 | |
| EMOS | 1.027 | 0.078 | 0.006 | 1.029 | 0.093 | 0.006 |

## CRPS skill score (cross-validation, reference: EMOS)

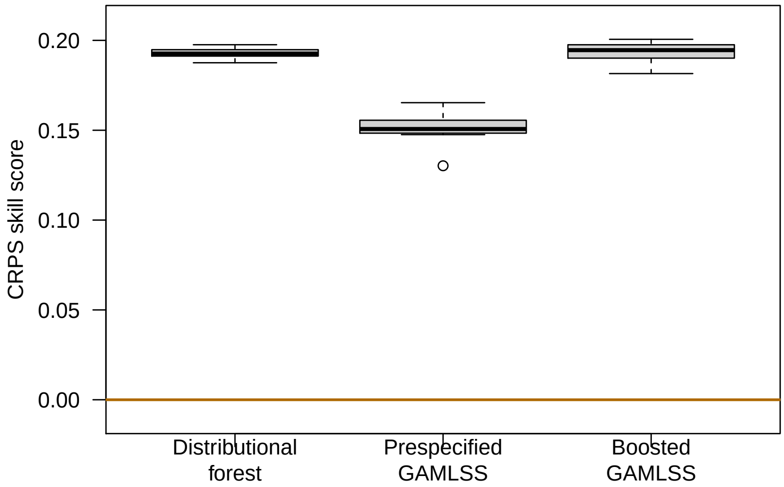


## Variable importance

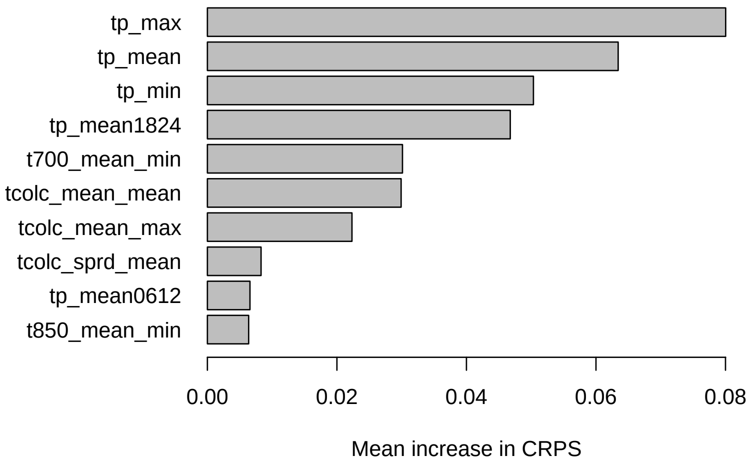

## Residual QQ plots

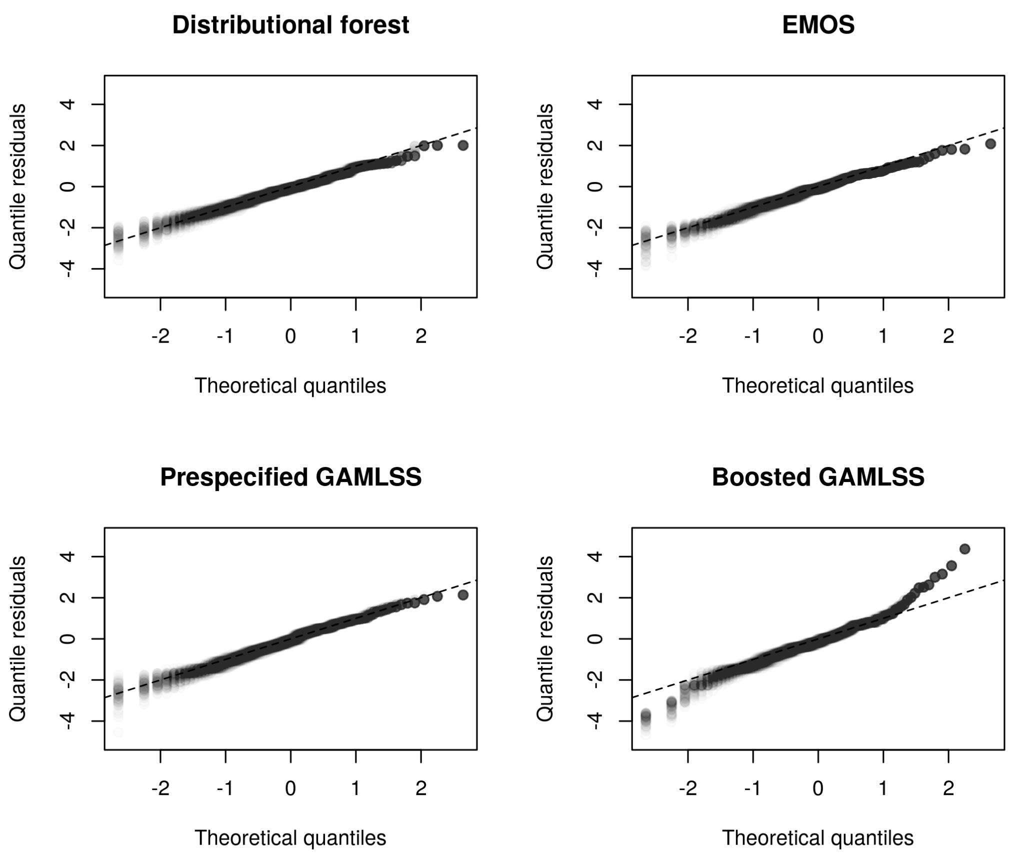


## PIT histograms

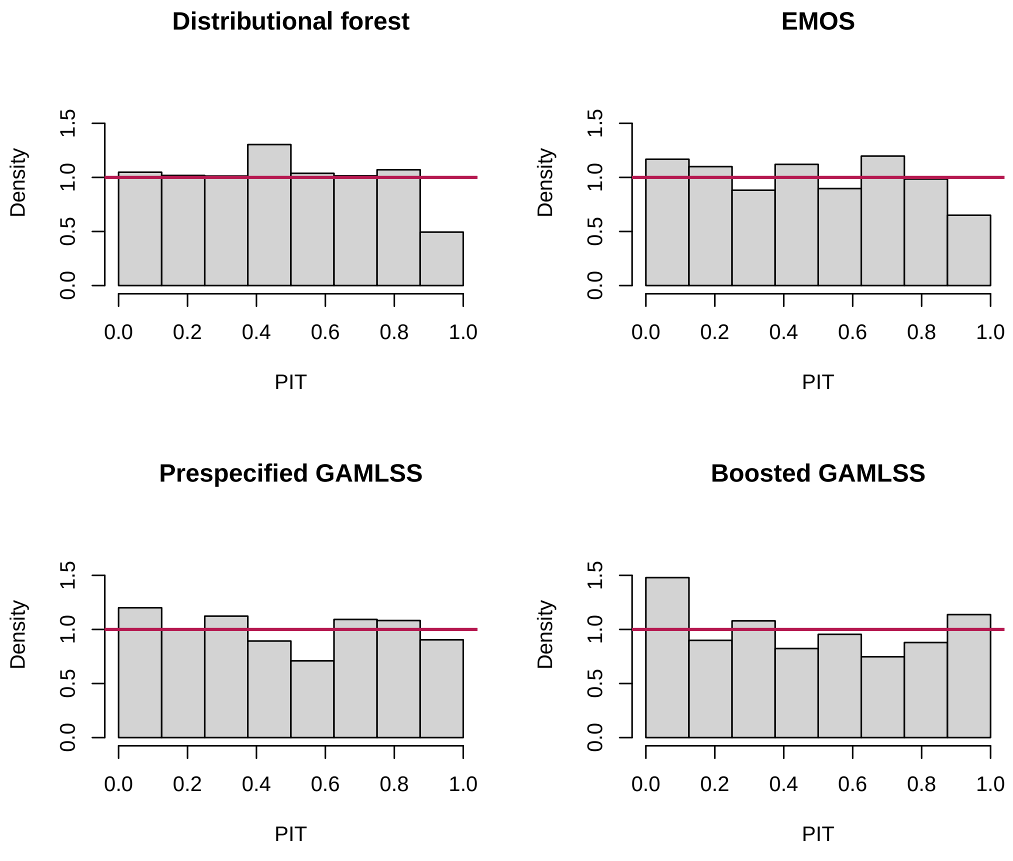

# See im Paznaun

Longitude: 10.465
Latitude: 47.084
Altitude: 1040.000

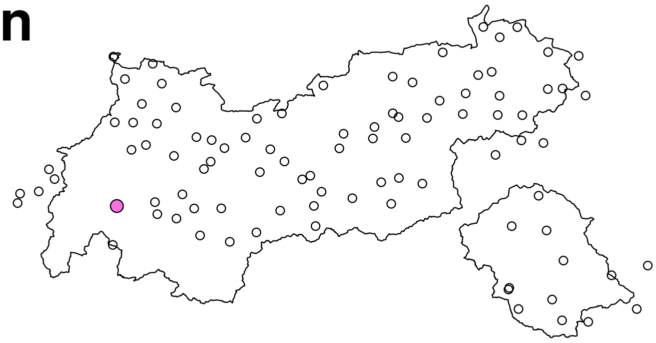

## Overview

| Model | Single split CRPS | Fit time | Predict time | 10 times 7-fold cross-validation CRPS | Fit time | Predict time |
|---|---|---|---|---|---|---|
| Distributional forest | 0.669 | 70.744 | 0.314 | 0.646 | 78.744 | 4.239 |
| Prespecified GAMLSS | 0.688 | 98.390 | 0.270 | 0.666 | 121.797 | 0.376 |
| Boosted GAMLSS | 0.714 | 110.635 | 0.099 | 0.659 | 131.831 | 0.131 |
| *(mstop selection)* | | 1438.971 | | | 2373.859 | |
| EMOS | 0.778 | 0.084 | 0.006 | 0.727 | 0.091 | 0.005 |

## CRPS skill score (cross-validation, reference: EMOS)

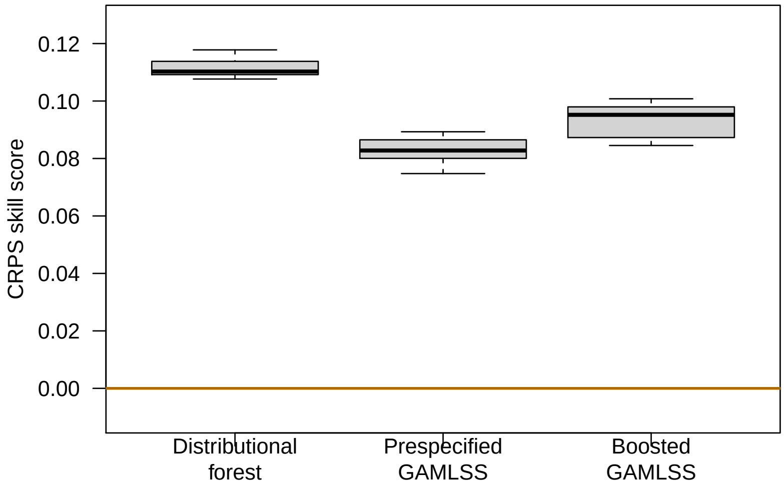


## Variable importance

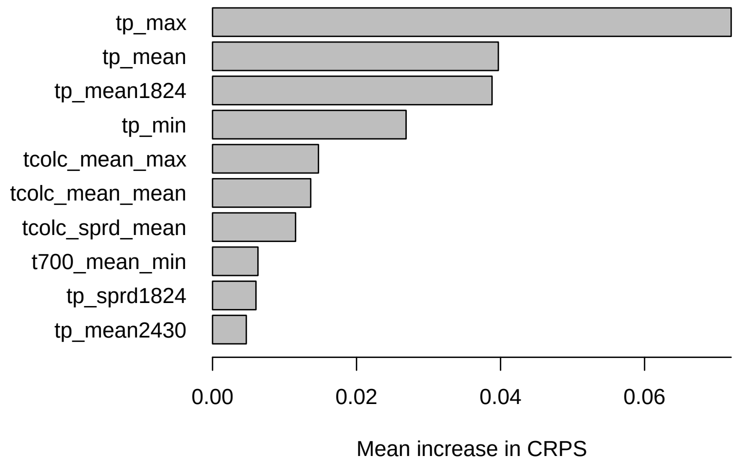

## Residual QQ plots

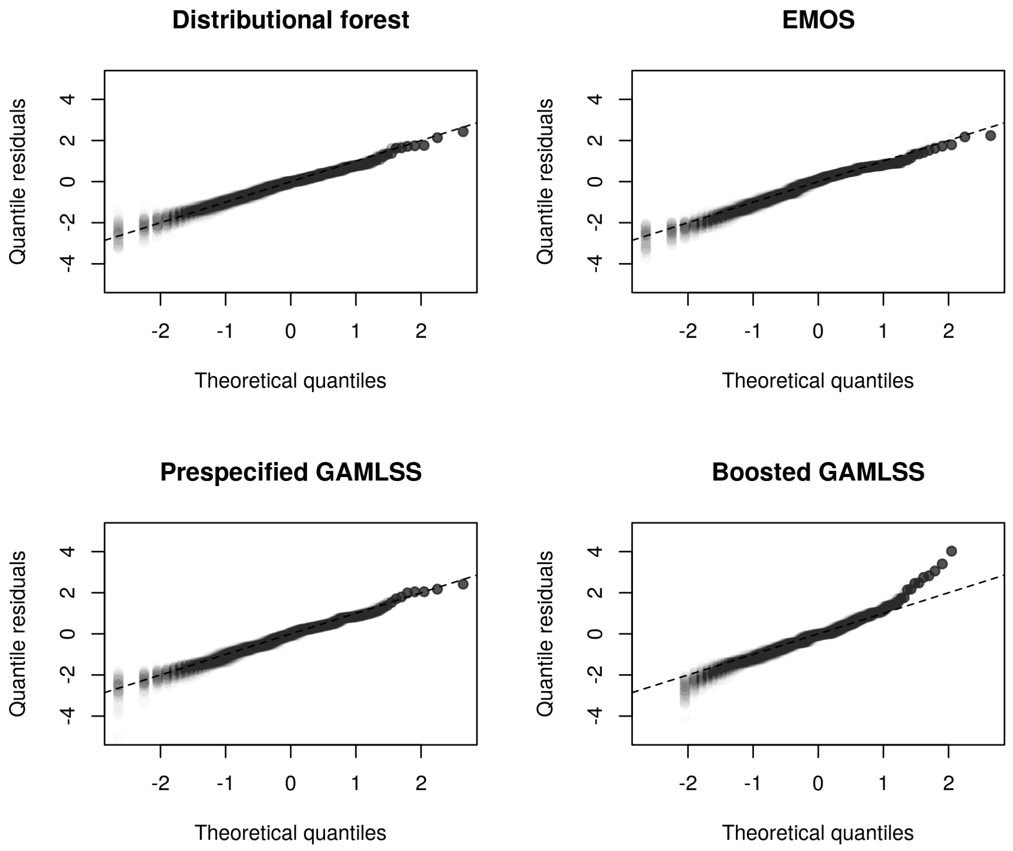


## PIT histograms

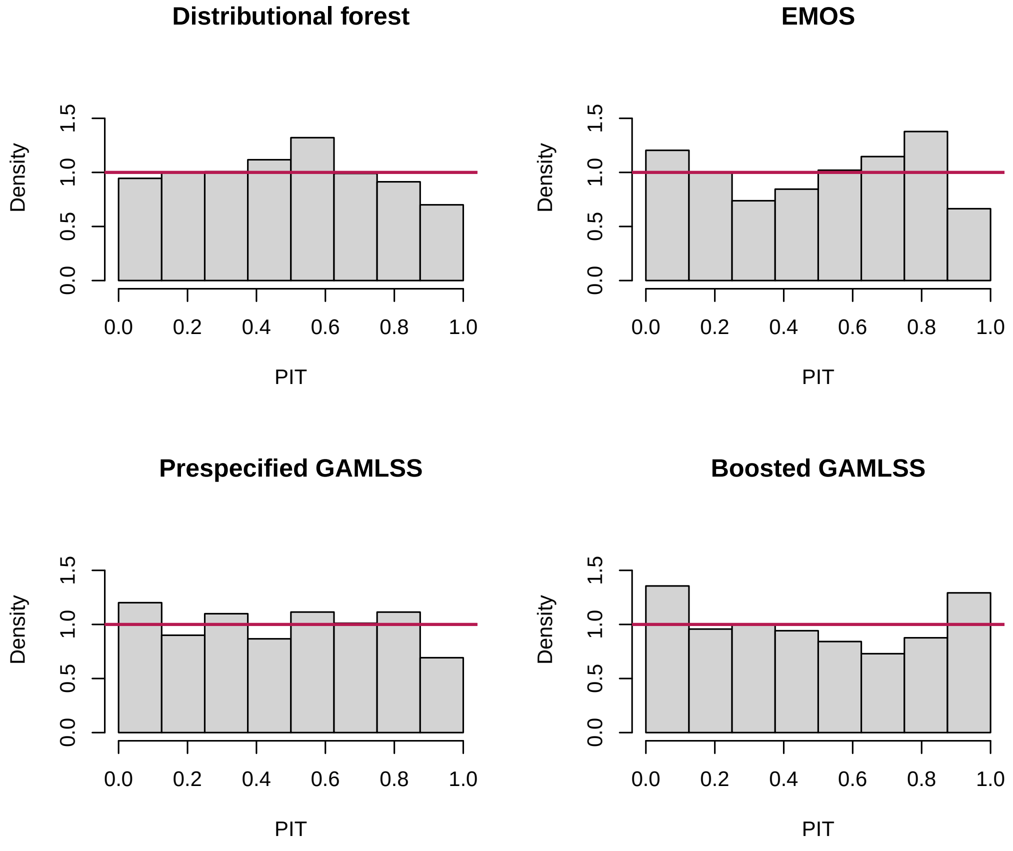

# Jungholz

Longitude: 10.448
Latitude: 47.575
Altitude: 1060.000

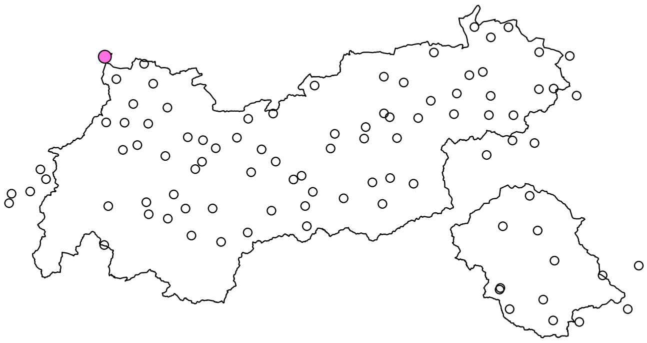

## Overview

| | Single split | | | 10 times 7-fold cross-validation | | |
|---|---|---|---|---|---|---|
| Model | CRPS | Fit time | Predict time | CRPS | Fit time | Predict time |
| Distributional forest | 0.779 | 70.203 | 0.302 | 0.903 | 78.919 | 4.527 |
| Prespecified GAMLSS | 0.749 | 210.053 | 0.263 | 0.913 | 182.050 | 0.370 |
| Boosted GAMLSS | 0.754 | 107.311 | 0.096 | 0.919 | 129.337 | 0.131 |
| *(mstop selection)* | | 1409.005 | | | 2325.032 | |
| EMOS | 0.914 | 0.083 | 0.006 | 1.011 | 0.090 | 0.005 |

## CRPS skill score (cross-validation, reference: EMOS)

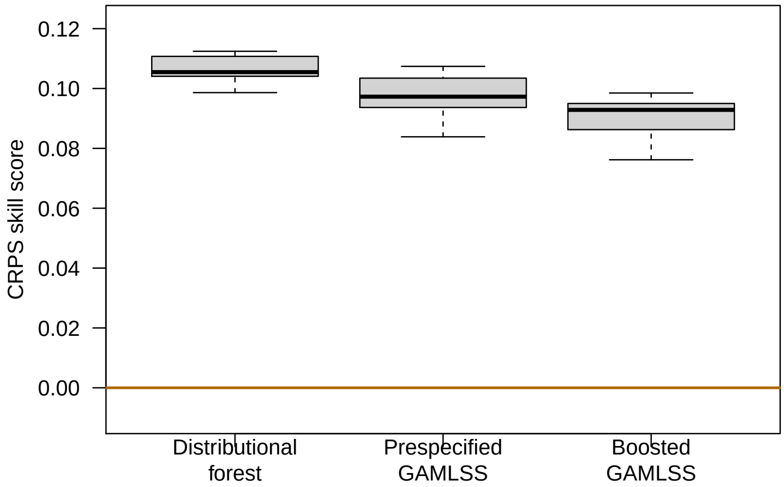


## Variable importance

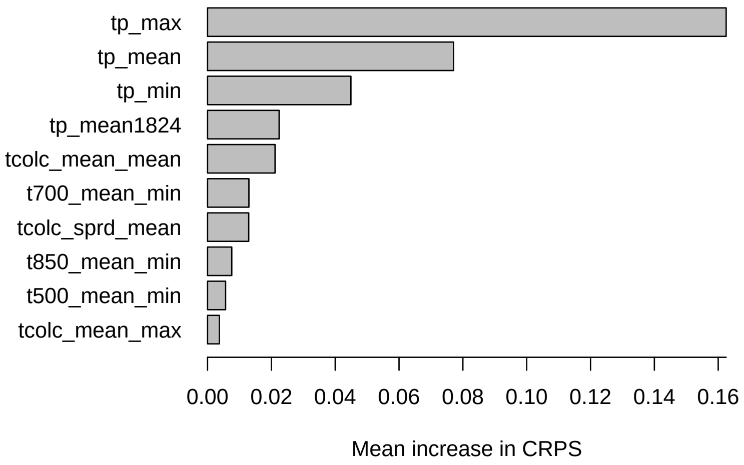

## Residual QQ plots

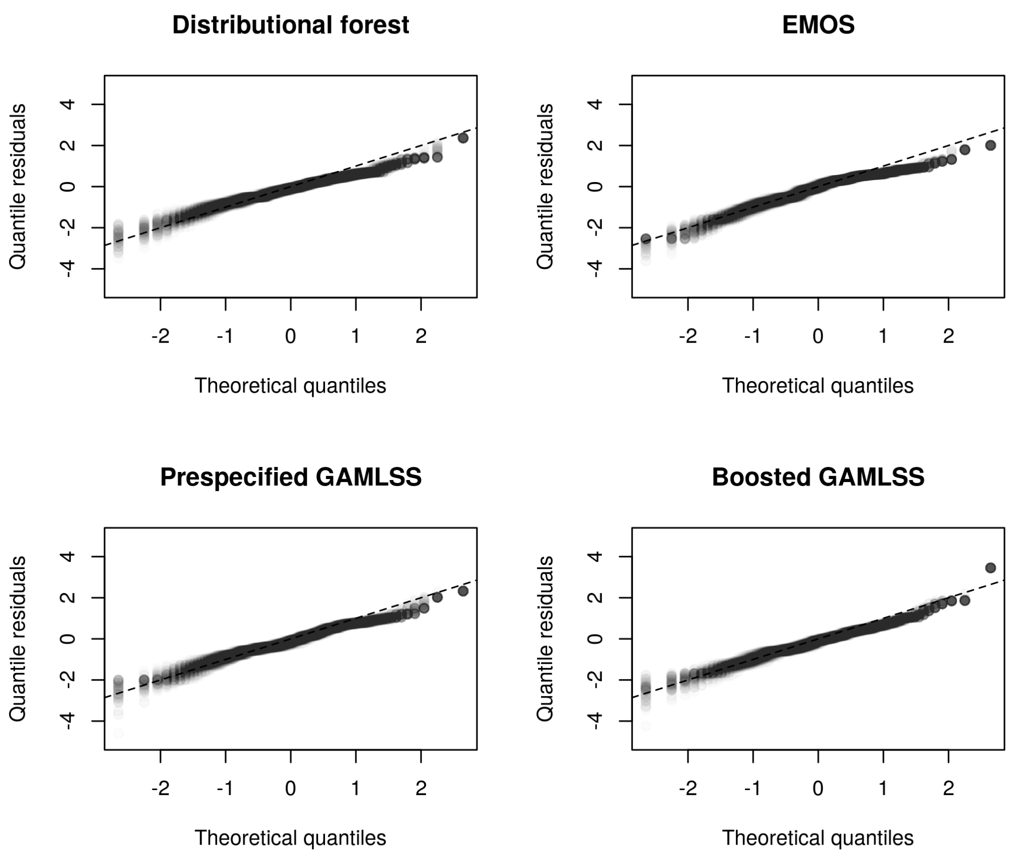


## PIT histograms

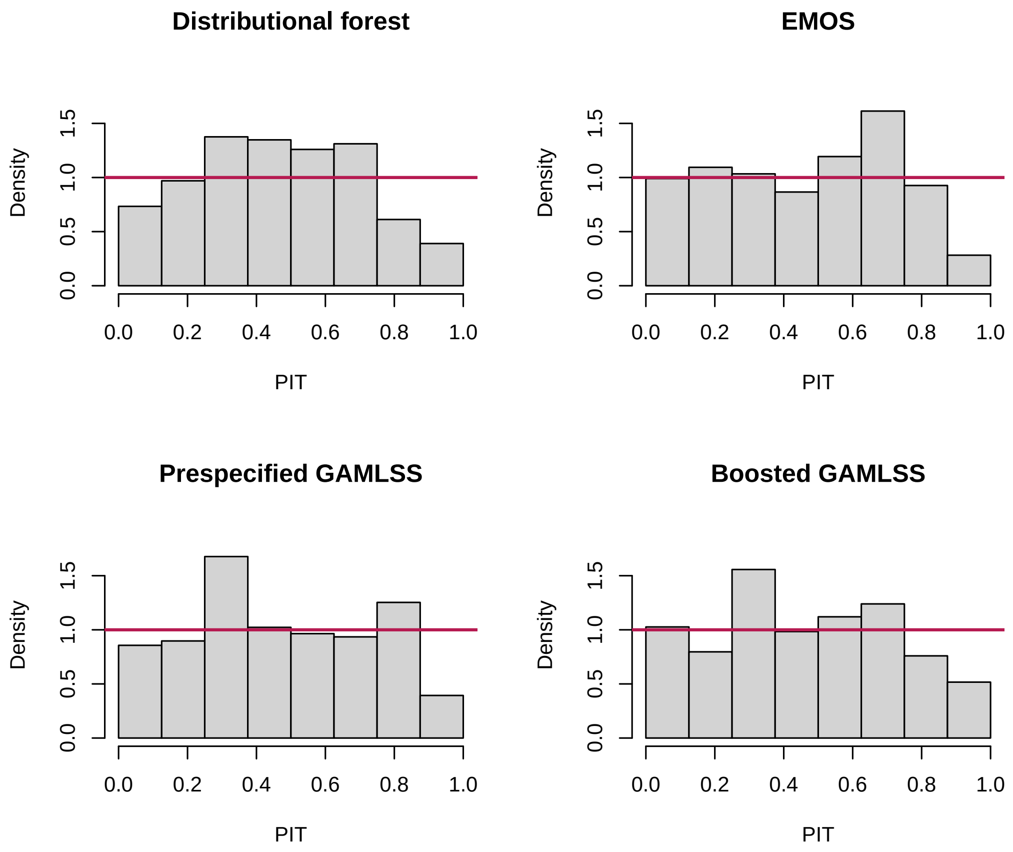

# Ladis-Neuegg

Longitude: 10.649
Latitude: 47.097
Altitude: 1350.000

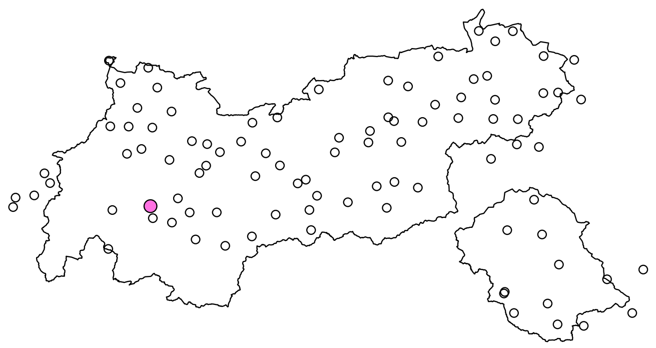

### Overview

| | Single split | | | 10 times 7-fold cross-validation | | |
|---|---|---|---|---|---|---|
| Model | CRPS | Fit time | Predict time | CRPS | Fit time | Predict time |
| Distributional forest | 0.802 | 70.644 | 0.315 | 0.672 | 77.555 | 4.148 |
| Prespecified GAMLSS | 0.806 | 87.272 | 0.249 | 0.667 | 98.883 | 0.369 |
| Boosted GAMLSS | 0.820 | 111.267 | 0.080 | 0.671 | 132.437 | 0.129 |
| *(mstop selection)* | | 1447.377 | | | 2392.028 | |
| EMOS | 0.828 | 0.083 | 0.006 | 0.707 | 0.094 | 0.005 |

### CRPS skill score (cross-validation, reference: EMOS)

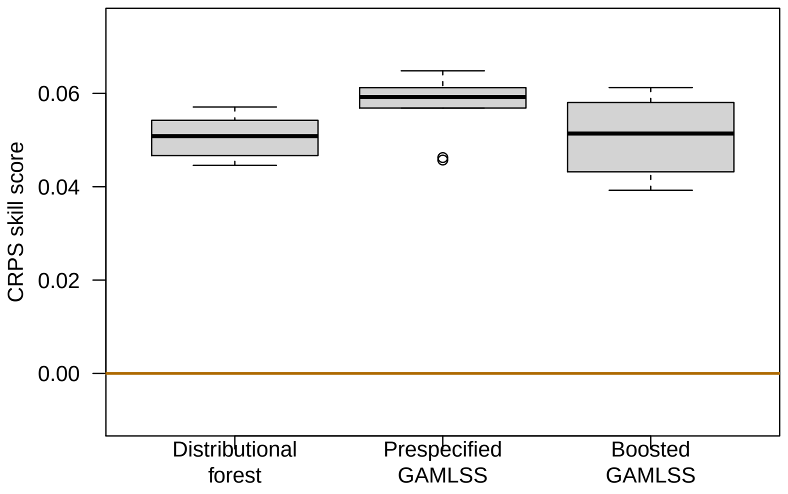


### Variable importance

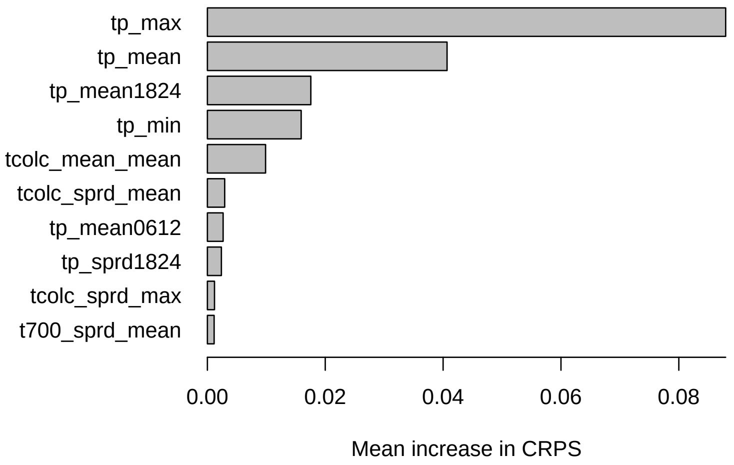

## Residual QQ plots

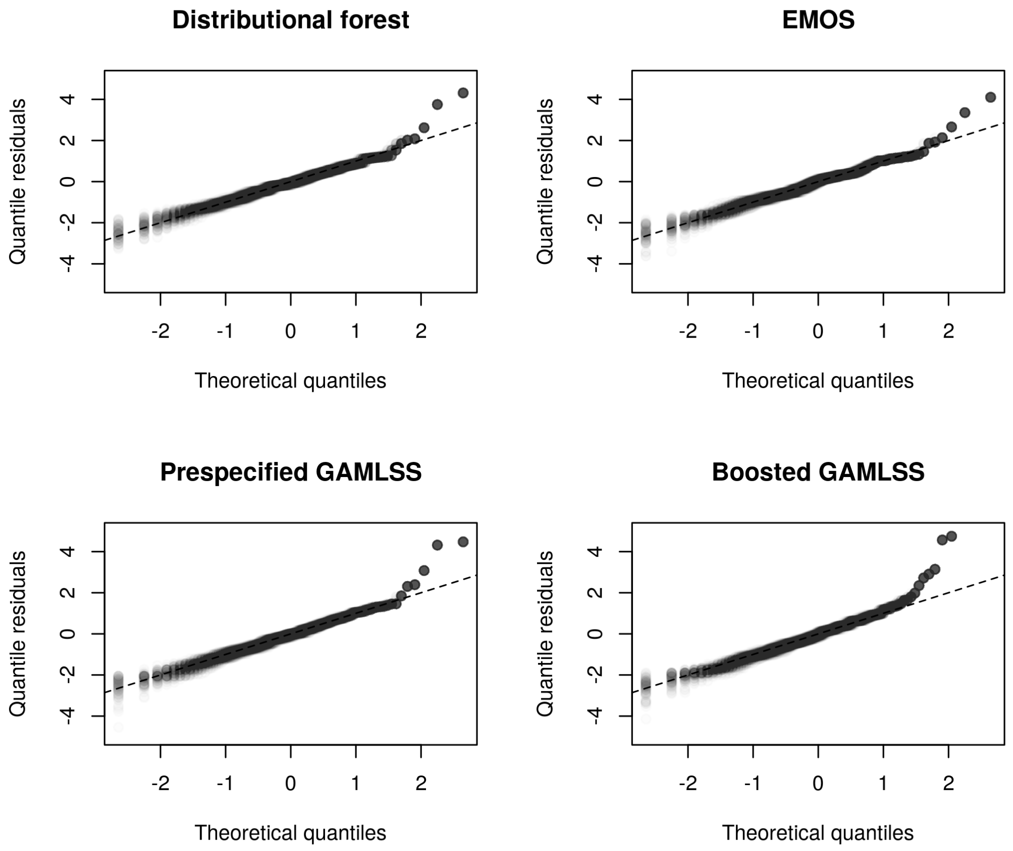


## PIT histograms

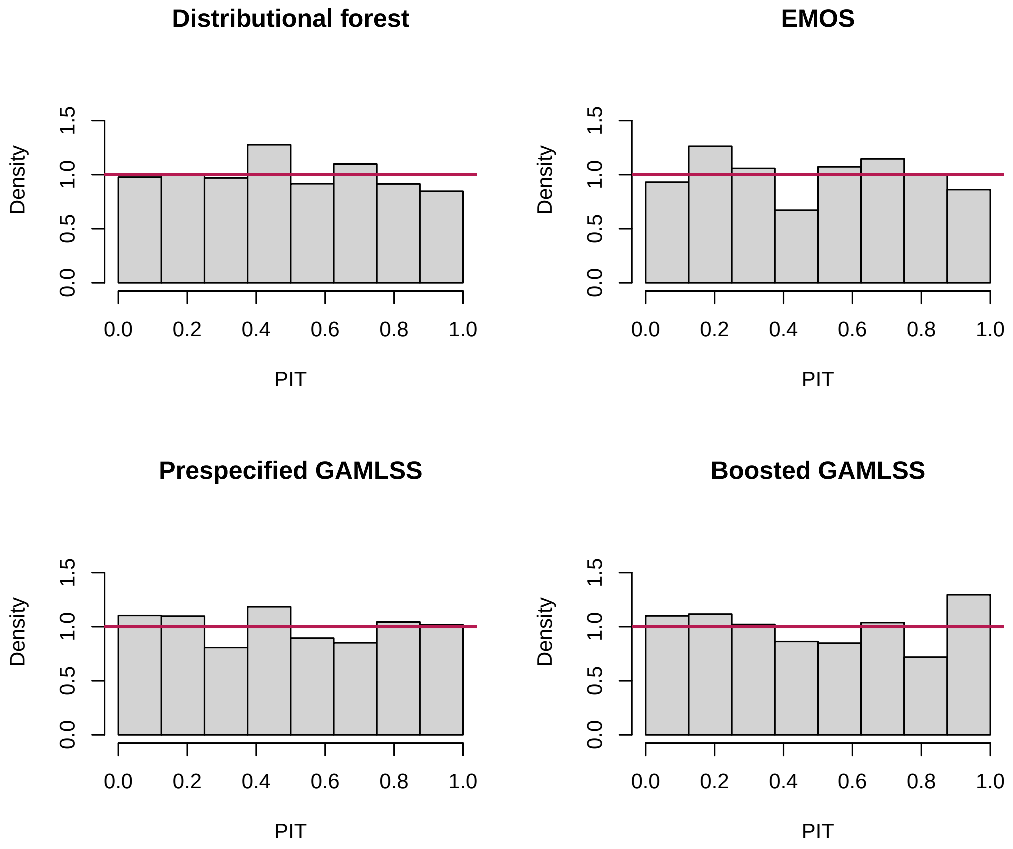

# Oetz

Longitude: 10.886
Latitude: 47.206
Altitude: 760.000

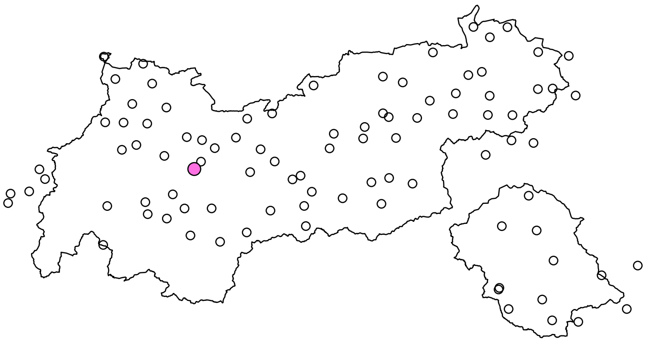

## Overview

| Model | Single split CRPS | Single split Fit time | Single split Predict time | 10 times 7-fold cross-validation CRPS | 10 times 7-fold cross-validation Fit time | 10 times 7-fold cross-validation Predict time |
|---|---|---|---|---|---|---|
| Distributional forest | 0.702 | 71.825 | 0.316 | 0.626 | 79.840 | 4.418 |
| Prespecified GAMLSS | 0.712 | 104.301 | 0.269 | 0.637 | 94.586 | 0.394 |
| Boosted GAMLSS | 0.704 | 116.980 | 0.121 | 0.630 | 132.723 | 0.145 |
| *(mstop selection)* | | 1449.459 | | | 2370.643 | |
| EMOS | 0.751 | 0.090 | 0.006 | 0.670 | 0.096 | 0.006 |

## CRPS skill score (cross-validation, reference: EMOS)

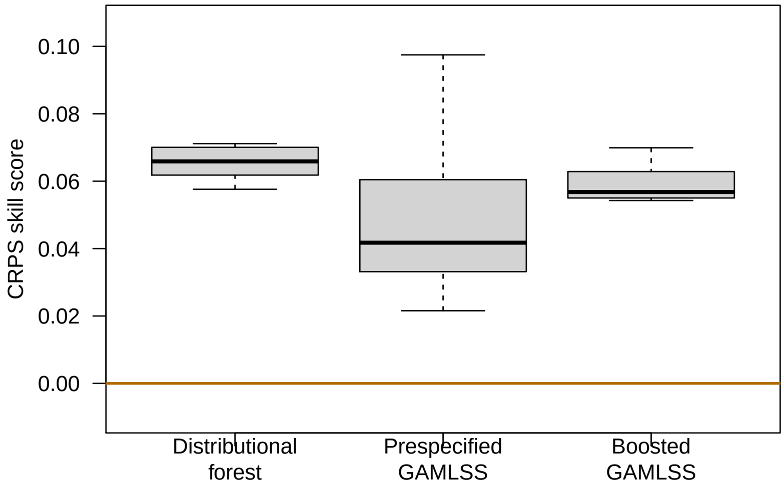


## Variable importance

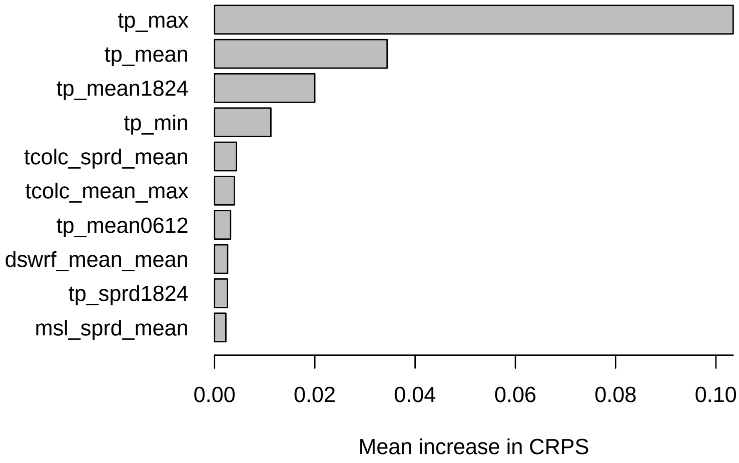

## Residual QQ plots

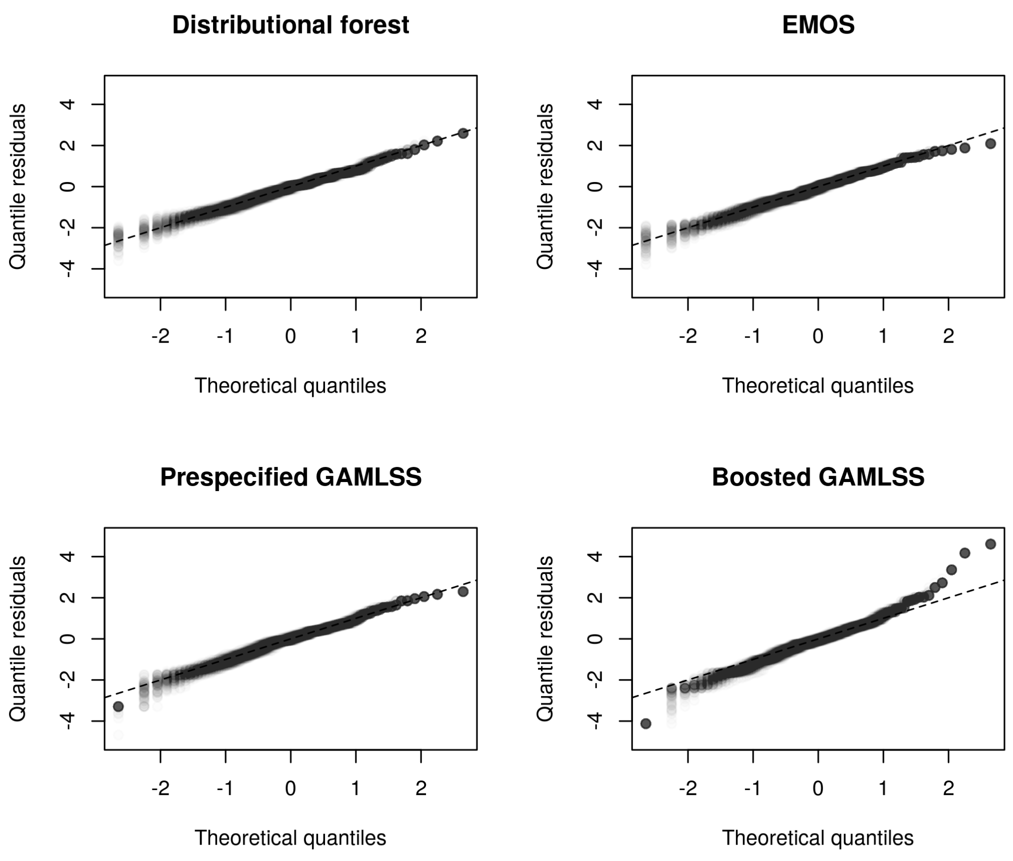


## PIT histograms

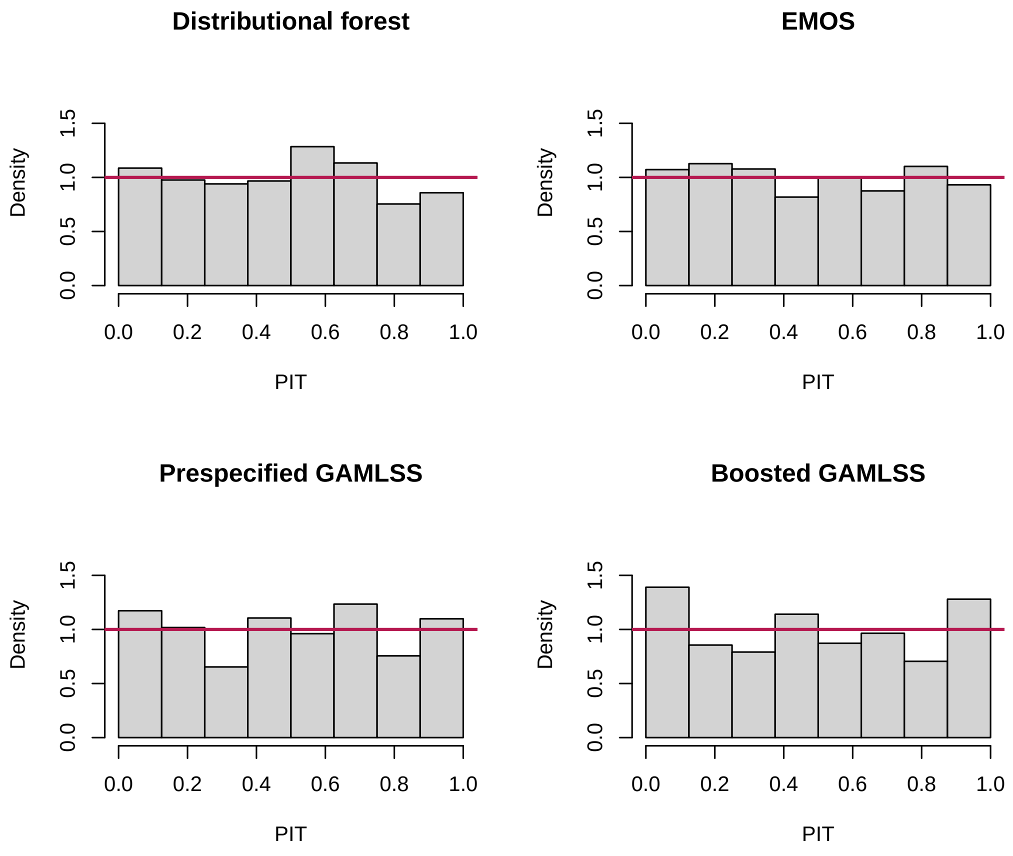

# Ochsengarten-Obergut

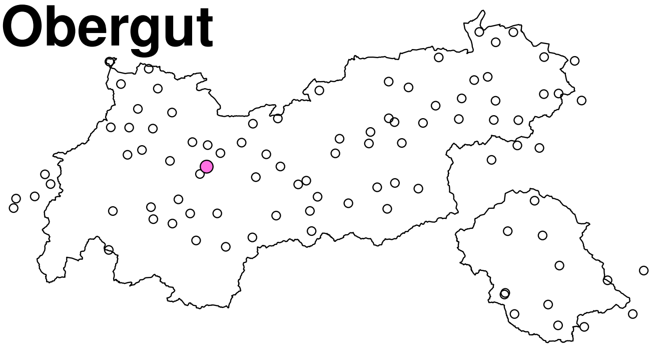

Longitude: 10.919
Latitude: 47.230
Altitude: 1695.000

## Overview

| | Single split | | | 10 times 7-fold cross-validation | | |
|---|---|---|---|---|---|---|
| Model | CRPS | Fit time | Predict time | CRPS | Fit time | Predict time |
| Distributional forest | 0.724 | 70.015 | 0.319 | 0.674 | 80.603 | 4.265 |
| Prespecified GAMLSS | 0.734 | 13.923 | 0.264 | 0.690 | 69.073 | 0.379 |
| Boosted GAMLSS | 0.697 | 110.400 | 0.104 | 0.685 | 132.588 | 0.135 |
| *(mstop selection)* | | 1443.430 | | | 2353.402 | |
| EMOS | 0.771 | 0.083 | 0.006 | 0.737 | 0.094 | 0.005 |

## CRPS skill score (cross-validation, reference: EMOS)

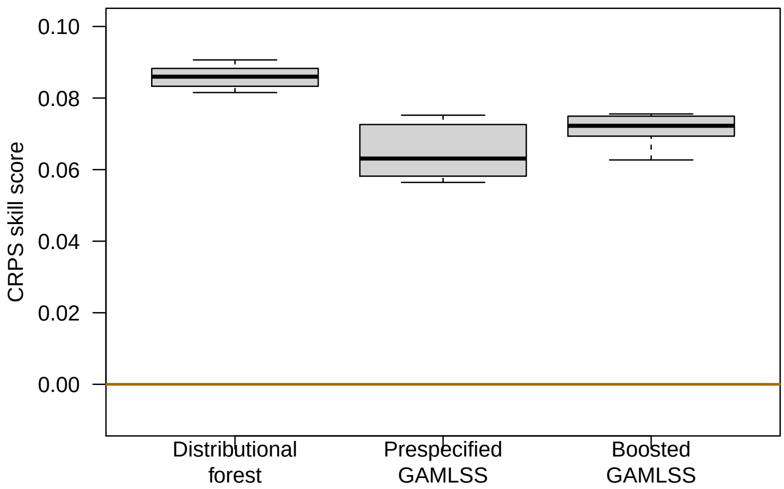


## Variable importance

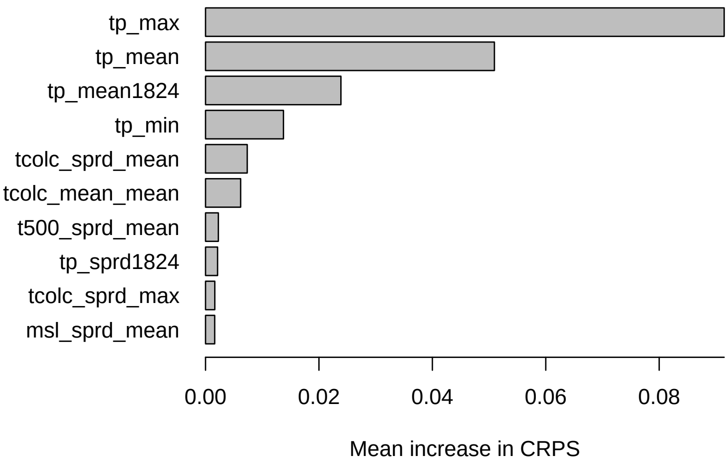

## Residual QQ plots

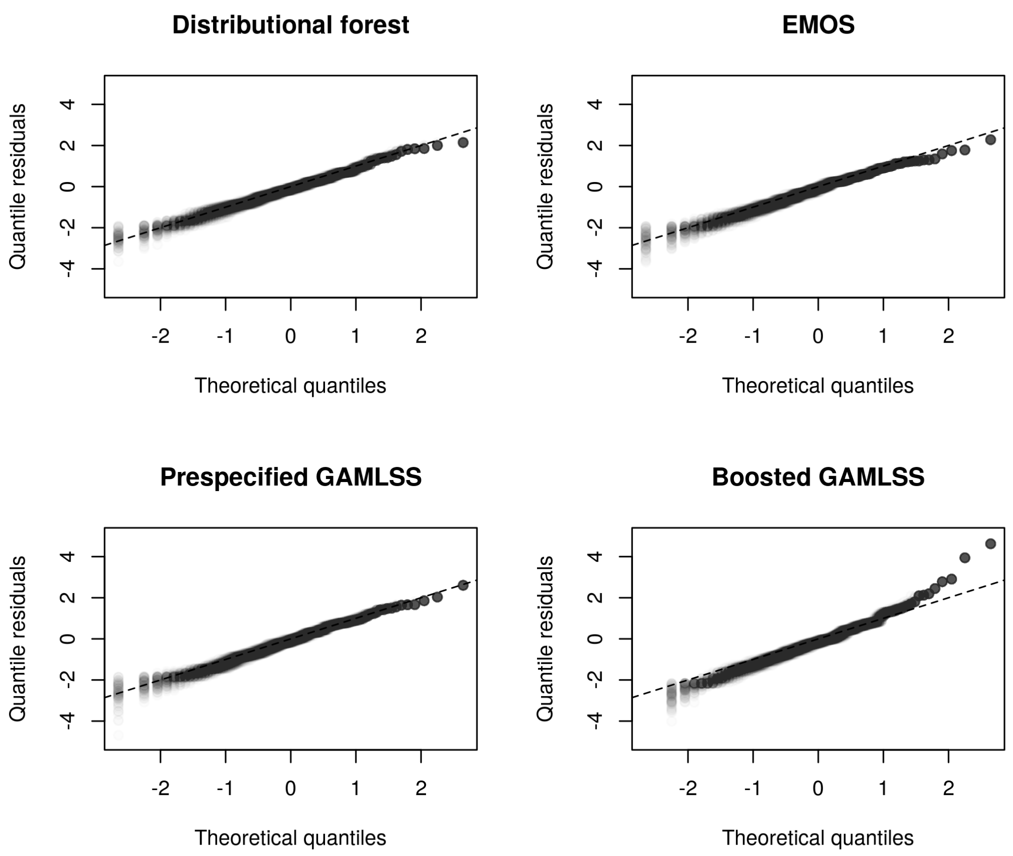


## PIT histograms

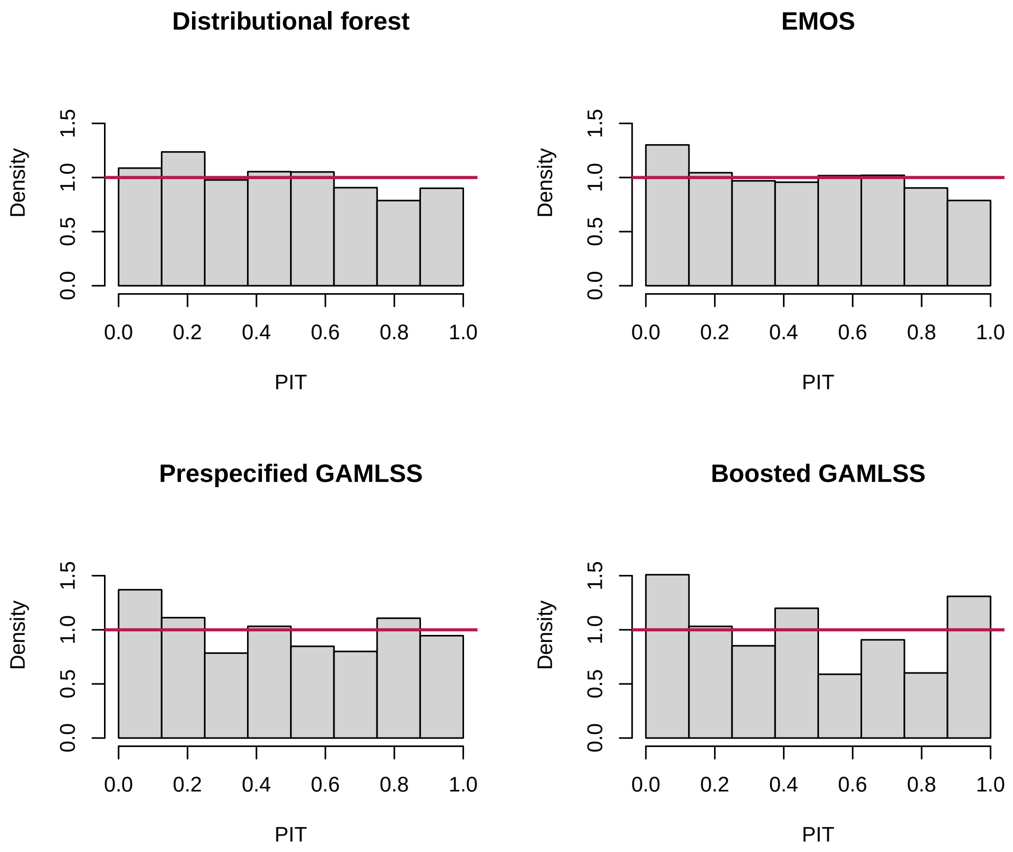

# Ginzling

Longitude: 11.793
Latitude: 47.091
Altitude: 1060.000

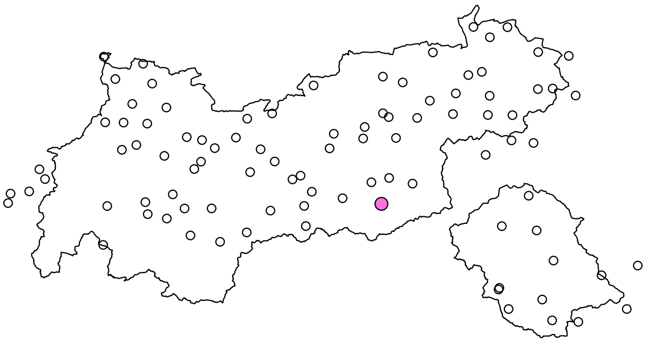

## Overview

| Model | Single split CRPS | Fit time | Predict time | 10 times 7-fold cross-validation CRPS | Fit time | Predict time |
|---|---|---|---|---|---|---|
| Distributional forest | 0.799 | 69.656 | 0.316 | 0.761 | 79.124 | 4.188 |
| Prespecified GAMLSS | 0.822 | 120.277 | 0.262 | 0.785 | 120.810 | 0.388 |
| Boosted GAMLSS | 0.818 | 111.684 | 0.113 | 0.787 | 132.579 | 0.150 |
| *(mstop selection)* | | 1426.743 | | | 2343.390 | |
| EMOS | 0.872 | 0.096 | 0.006 | 0.853 | 0.092 | 0.005 |

## CRPS skill score (cross-validation, reference: EMOS)

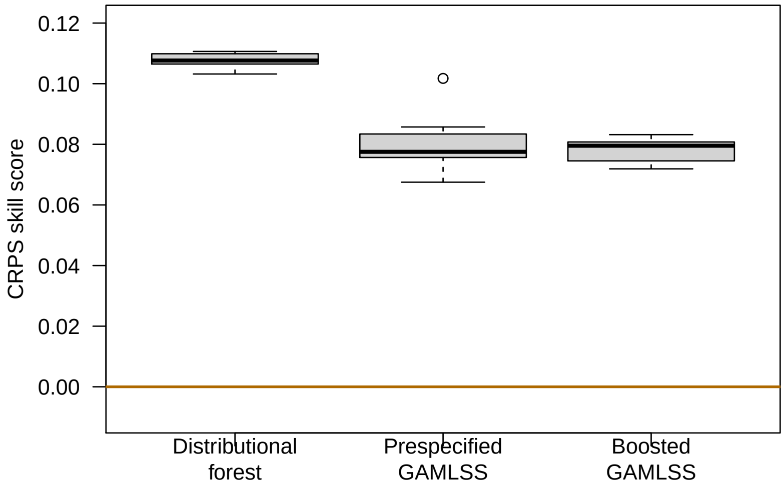


## Variable importance

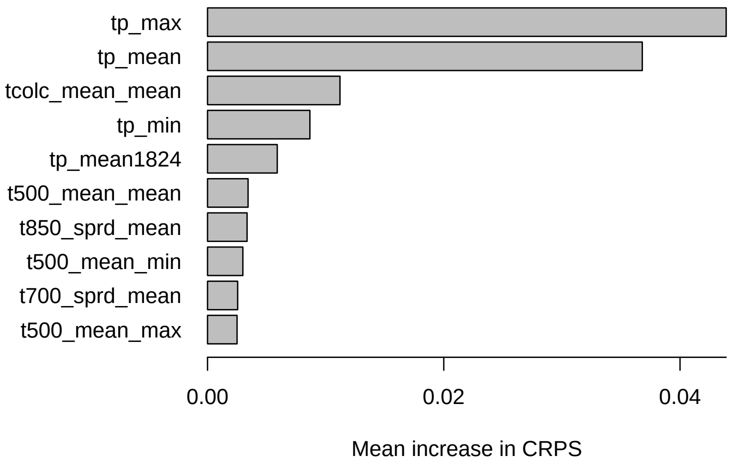

## Residual QQ plots

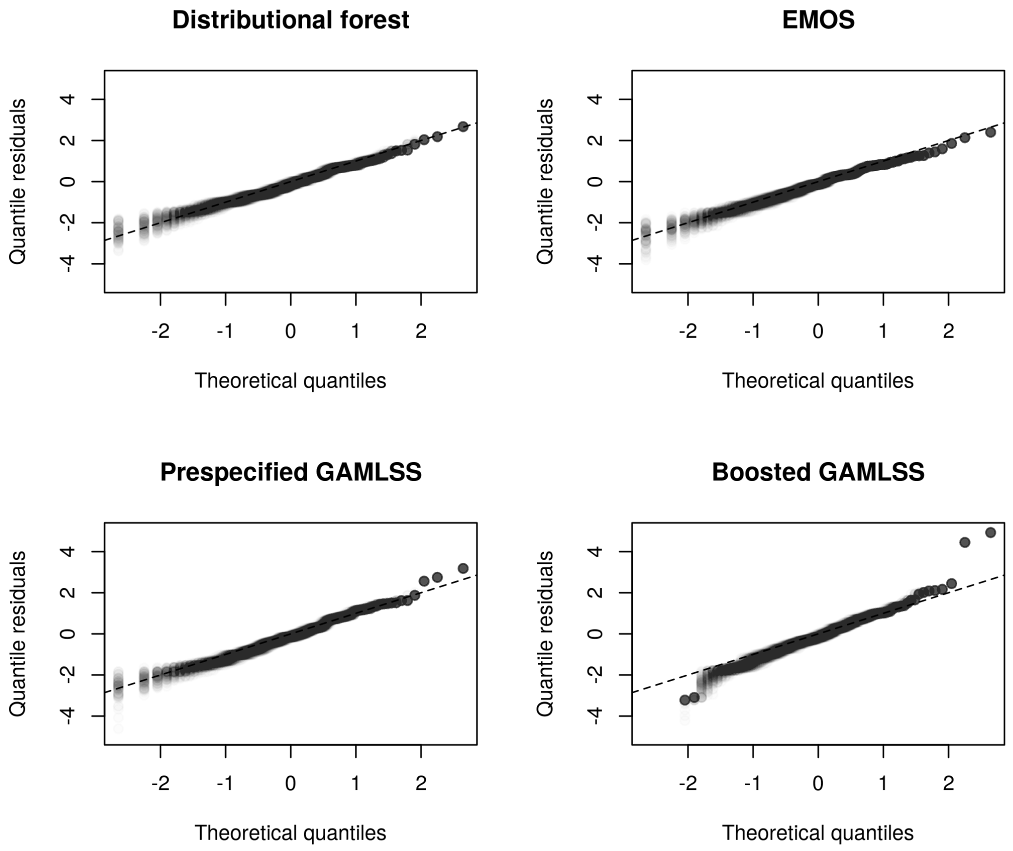


## PIT histograms

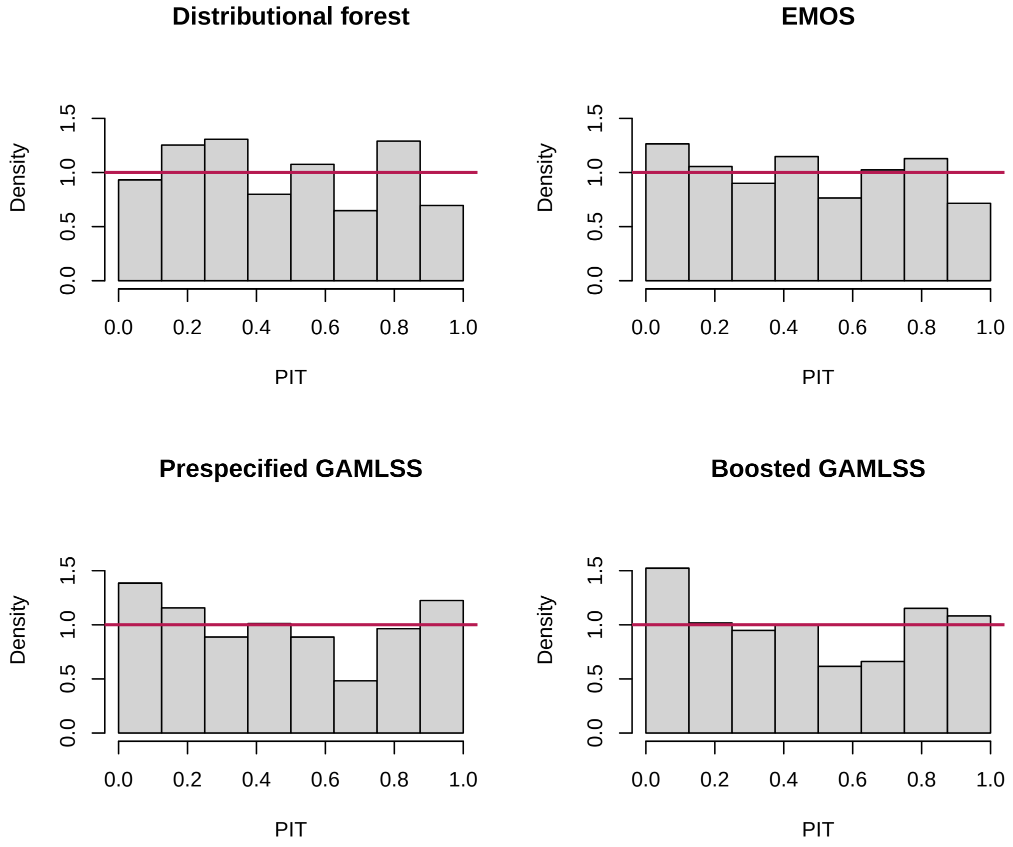

# Rotholz

Longitude: 11.800
Latitude: 47.389
Altitude: 563.000

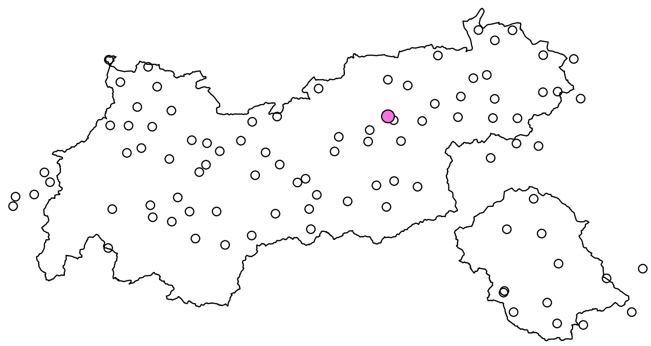

## Overview

| Model | Single split CRPS | Fit time | Predict time | 10 times 7-fold cross-validation CRPS | Fit time | Predict time |
|---|---|---|---|---|---|---|
| Distributional forest | 0.898 | 71.006 | 0.309 | 0.774 | 85.696 | 4.706 |
| Prespecified GAMLSS | 0.905 | 66.509 | 0.264 | 0.793 | 219.119 | 0.433 |
| Boosted GAMLSS | 0.939 | 111.320 | 0.093 | 0.786 | 134.582 | 0.142 |
| *(mstop selection)* | | 1417.318 | | | 2196.147 | |
| EMOS | 0.886 | 0.081 | 0.006 | 0.840 | 0.101 | 0.006 |

## CRPS skill score (cross-validation, reference: EMOS)

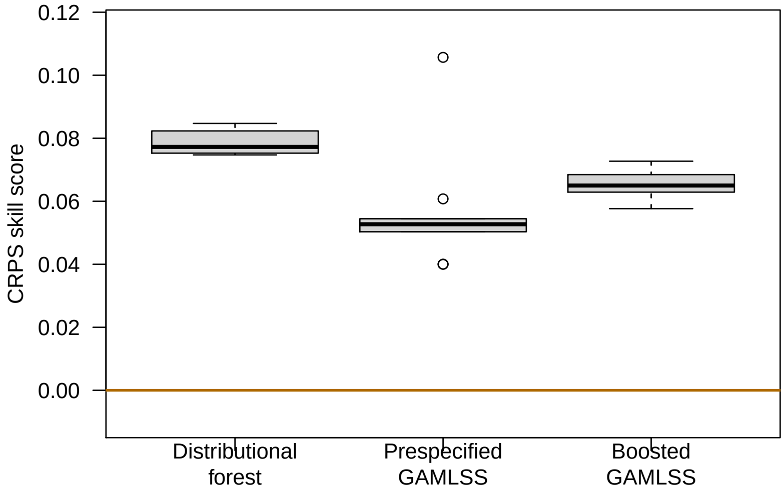


## Variable importance

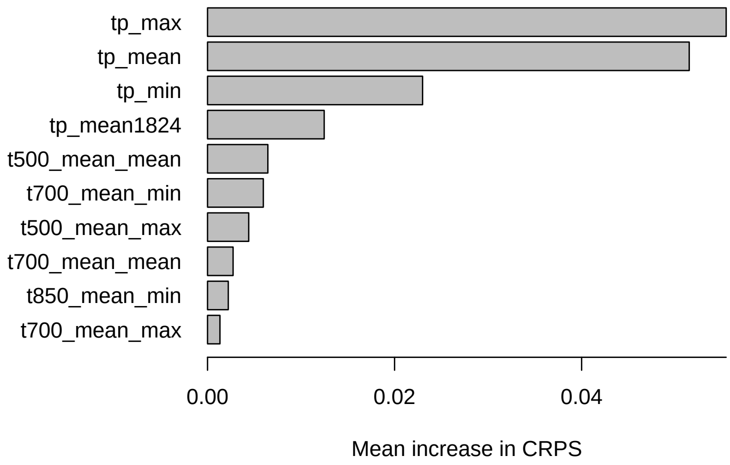

## Residual QQ plots

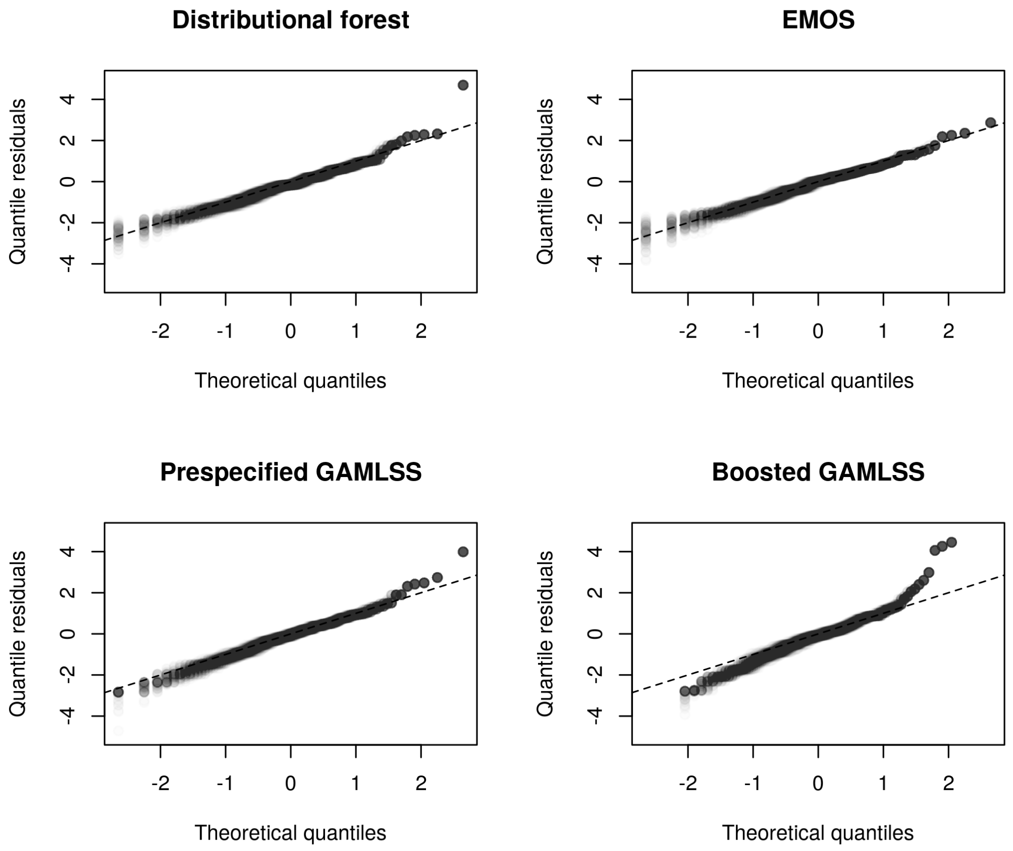


## PIT histograms

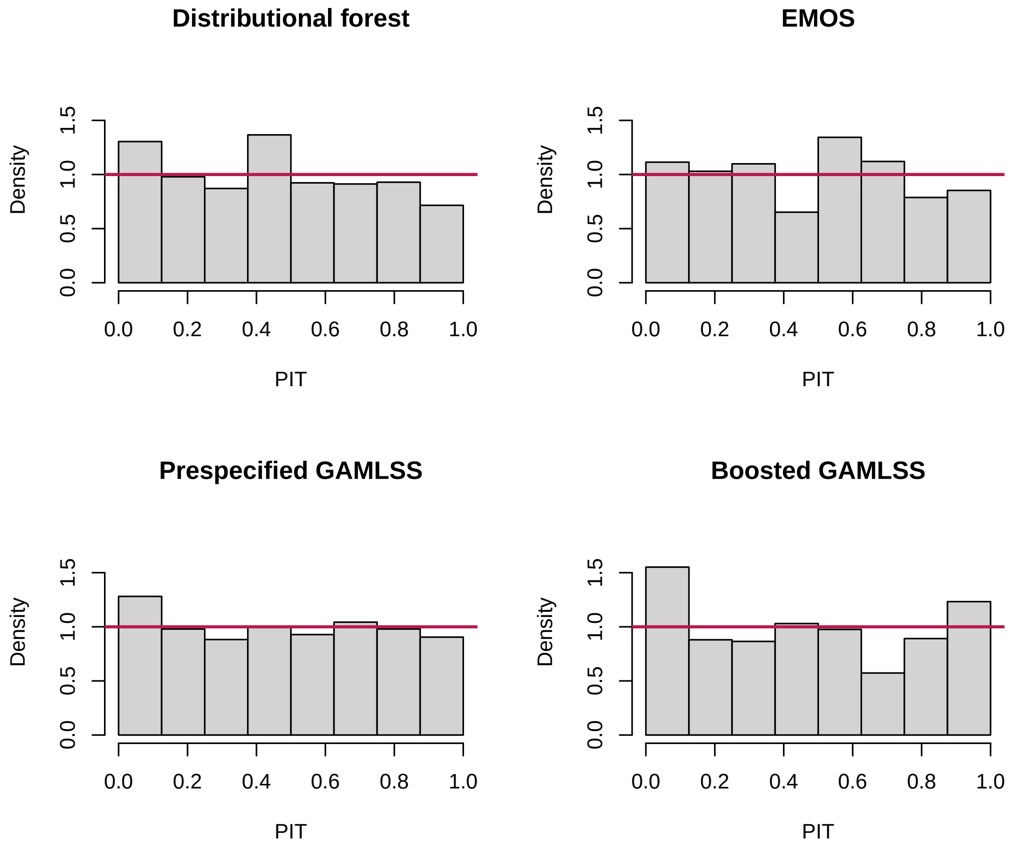

# Walchsee

Longitude: 12.318
Latitude: 47.639
Altitude: 687.000

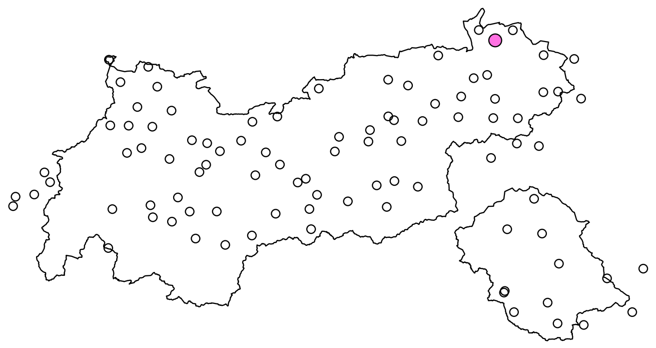

## Overview

| Model | Single split CRPS | Fit time | Predict time | 10 times 7-fold cross-validation CRPS | Fit time | Predict time |
|---|---|---|---|---|---|---|
| Distributional forest | 1.032 | 72.334 | 0.315 | 0.921 | 81.756 | 4.590 |
| Prespecified GAMLSS | 1.066 | 123.192 | 0.267 | 0.963 | 132.344 | 0.417 |
| Boosted GAMLSS | 1.082 | 108.411 | 0.092 | 0.940 | 131.766 | 0.133 |
| *(mstop selection)* | | 1401.731 | | | 2279.849 | |
| EMOS | 1.051 | 0.083 | 0.006 | 1.009 | 0.091 | 0.005 |

## CRPS skill score (cross-validation, reference: EMOS)

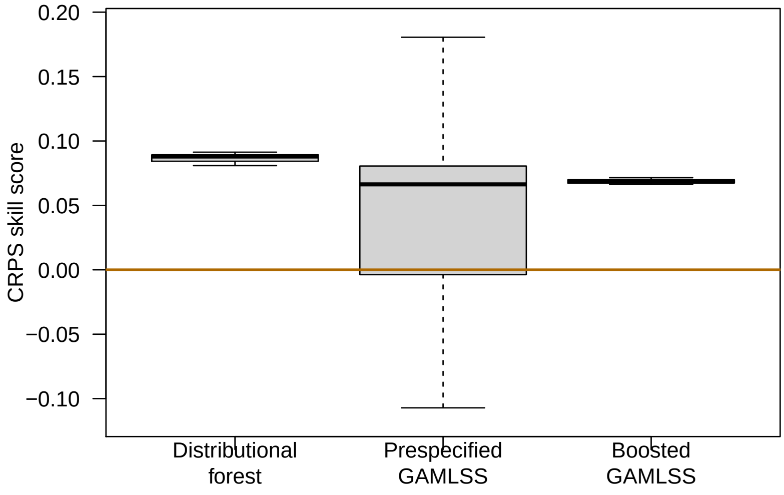


## Variable importance

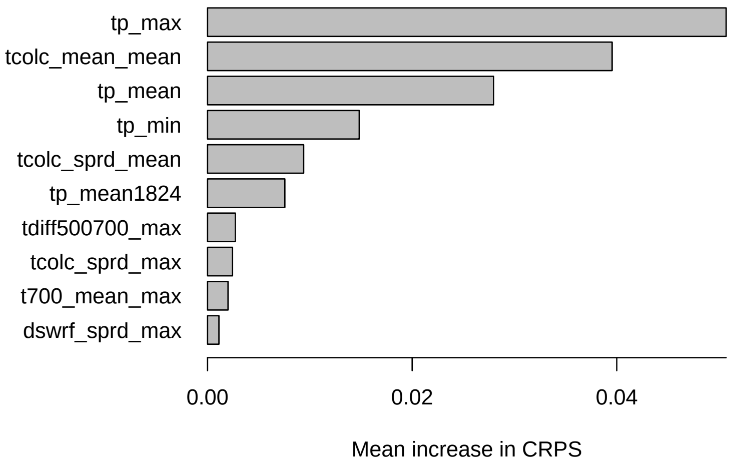

## Residual QQ plots

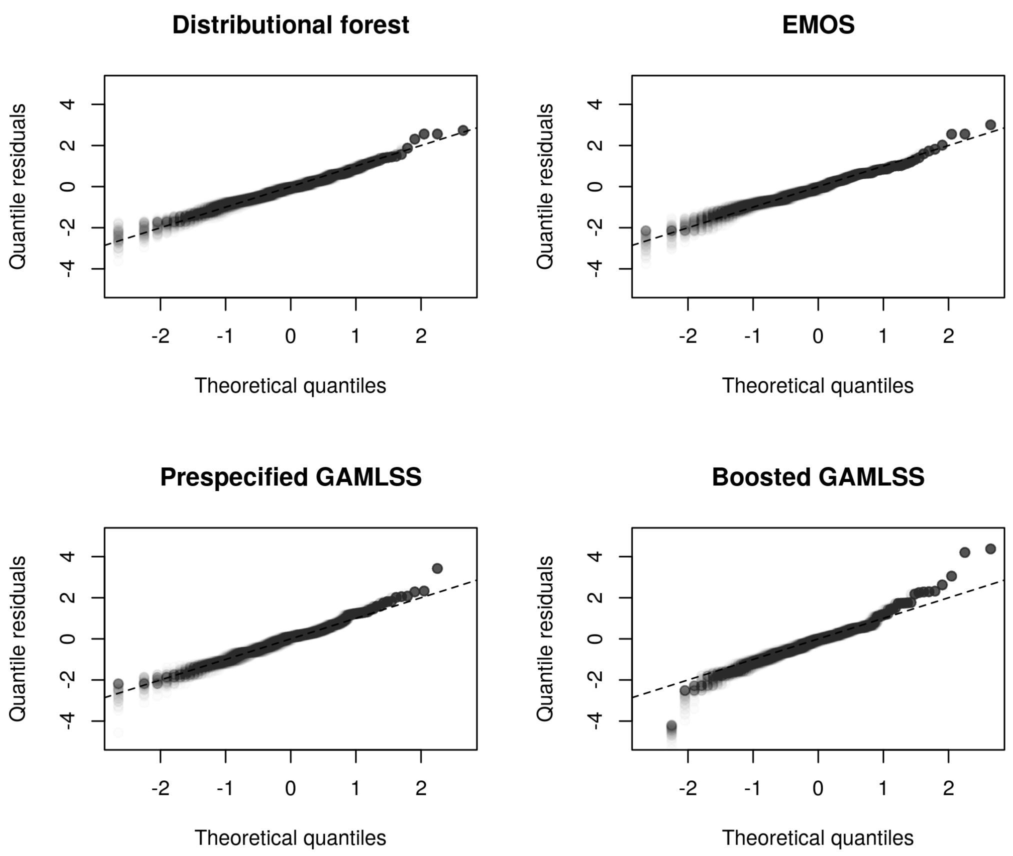


## PIT histograms

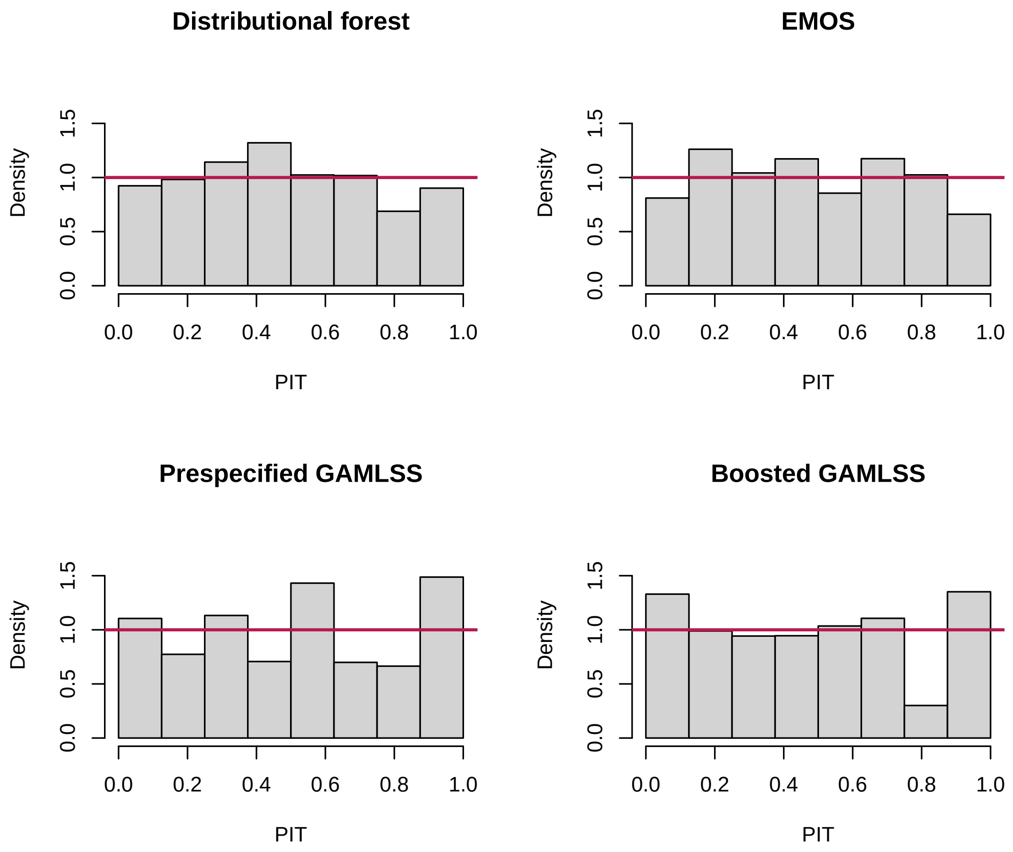

# Koessen

Longitude: 12.403
Latitude: 47.672
Altitude: 590.000

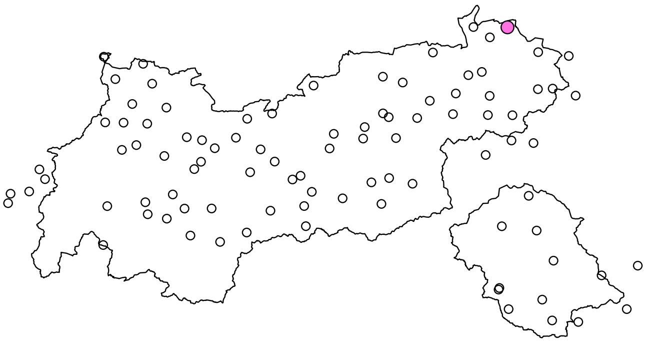

## Overview

| Model | Single split CRPS | Fit time | Predict time | 10 times 7-fold cross-validation CRPS | Fit time | Predict time |
|---|---|---|---|---|---|---|
| Distributional forest | 0.891 | 72.533 | 0.319 | 0.849 | 82.473 | 4.470 |
| Prespecified GAMLSS | 0.949 | 100.691 | 0.265 | 0.884 | 147.692 | 0.397 |
| Boosted GAMLSS | 0.917 | 109.716 | 0.095 | 0.862 | 131.997 | 0.143 |
| *(mstop selection)* | | 1419.662 | | | 2298.545 | |
| EMOS | 0.917 | 0.079 | 0.006 | 0.935 | 0.092 | 0.006 |

## CRPS skill score (cross-validation, reference: EMOS)

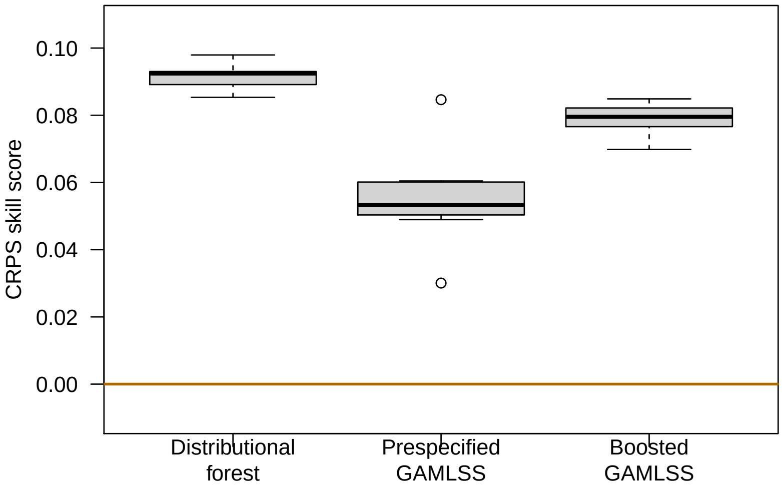


## Variable importance

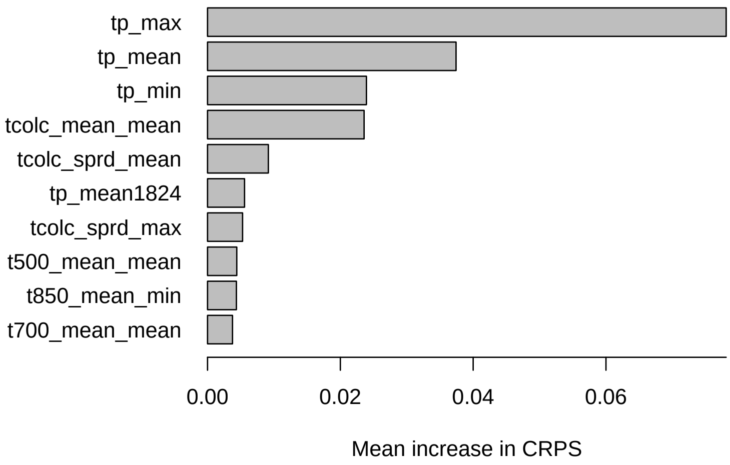

## Residual QQ plots

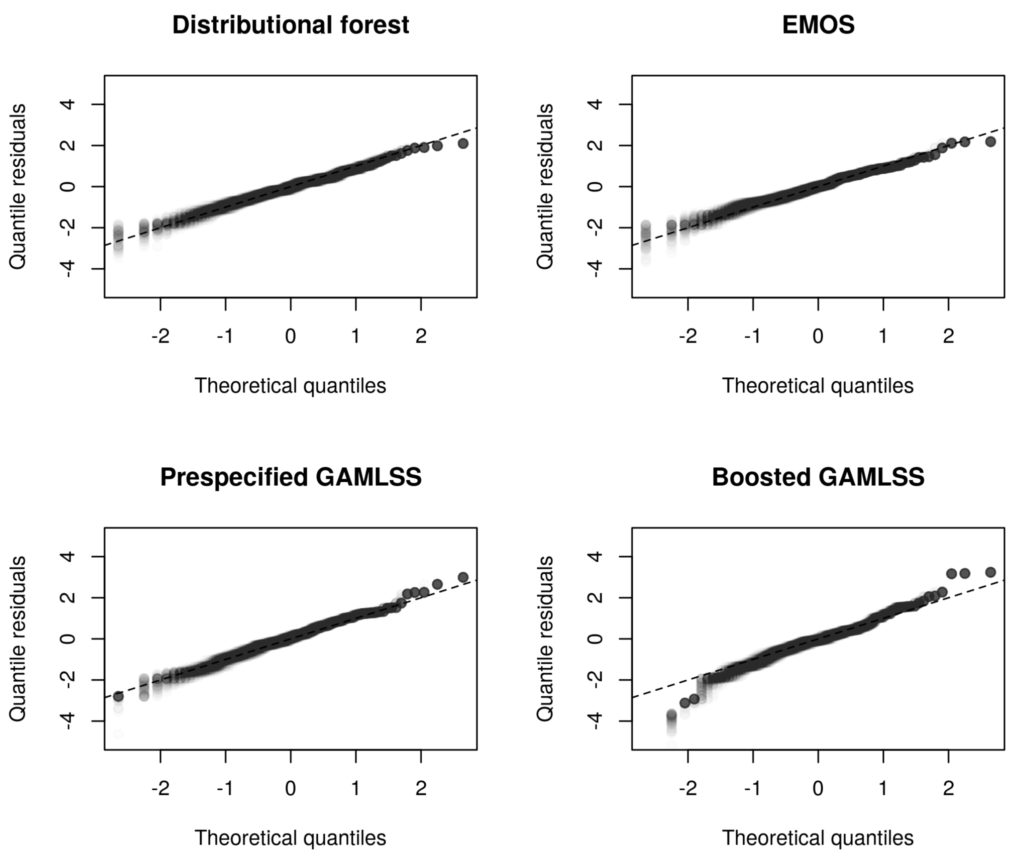


## PIT histograms

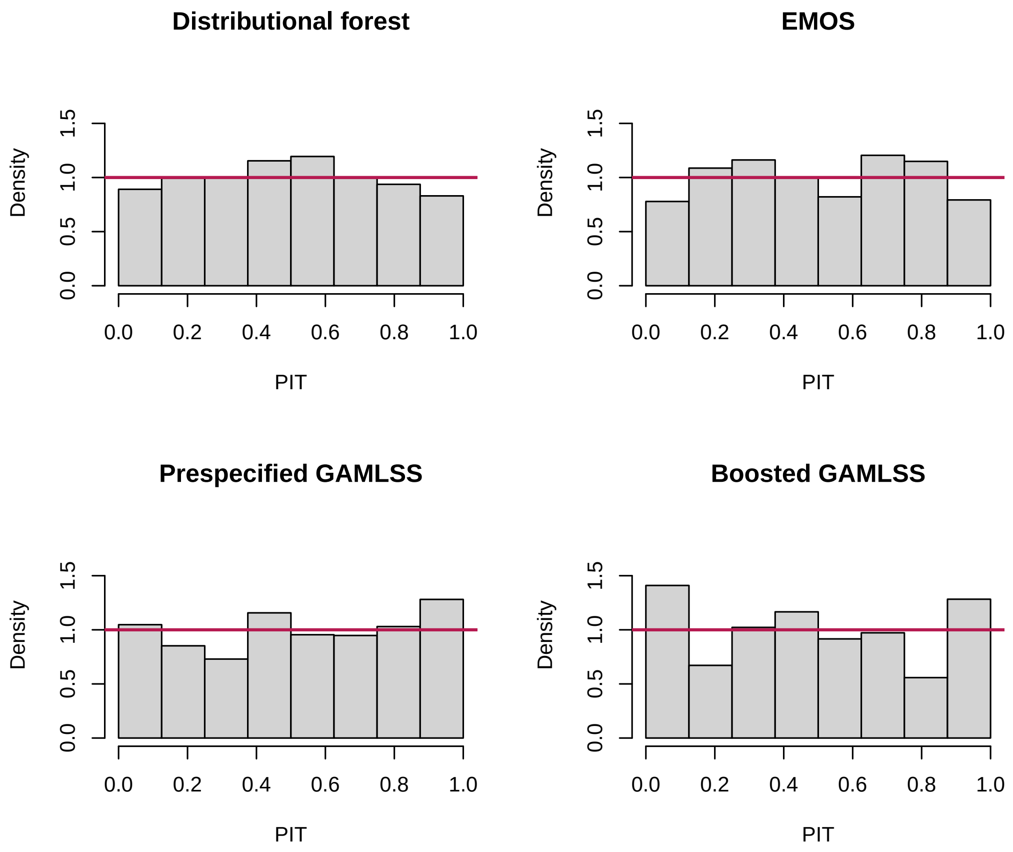

# Innervillgraten

Longitude: 12.360
Latitude: 46.810
Altitude: 1400.000

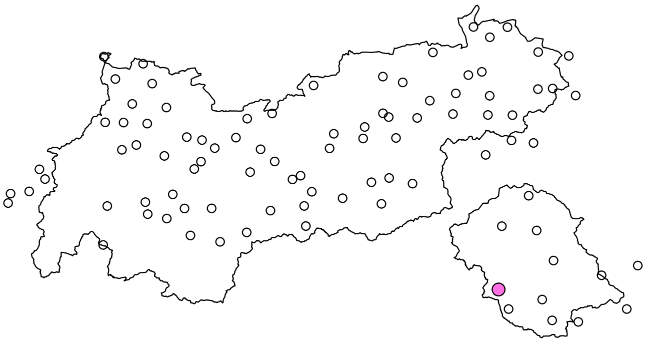

## Overview

| Model | Single split CRPS | Fit time | Predict time | 10 times 7-fold cross-validation CRPS | Fit time | Predict time |
|---|---|---|---|---|---|---|
| Distributional forest | 1.029 | 74.276 | 0.310 | 0.876 | 82.456 | 4.562 |
| Prespecified GAMLSS | 0.943 | 49.408 | 0.267 | 0.878 | 61.823 | 0.381 |
| Boosted GAMLSS | 1.008 | 110.858 | 0.097 | 0.894 | 129.667 | 0.126 |
| *(mstop selection)* | | 1403.836 | | | 2318.448 | |
| EMOS | 0.985 | 0.087 | 0.006 | 0.936 | 0.100 | 0.005 |

## CRPS skill score (cross-validation, reference: EMOS)

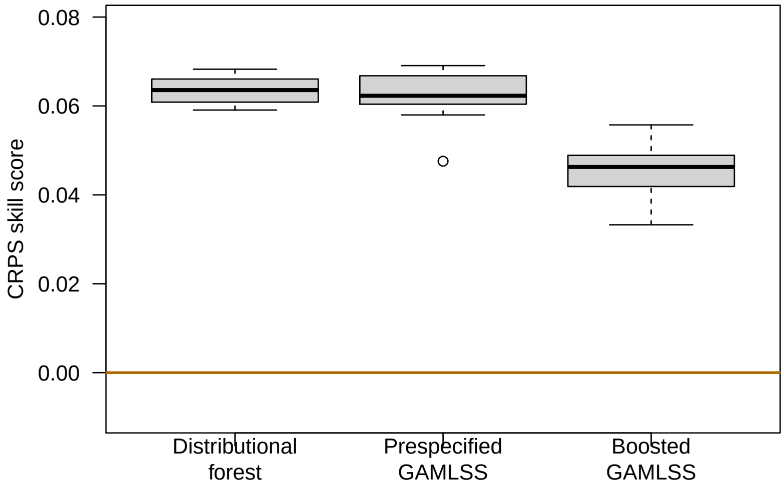


## Variable importance

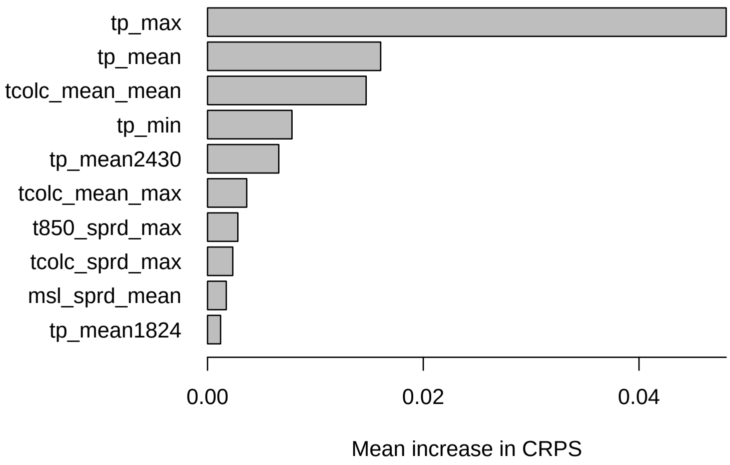

## Residual QQ plots

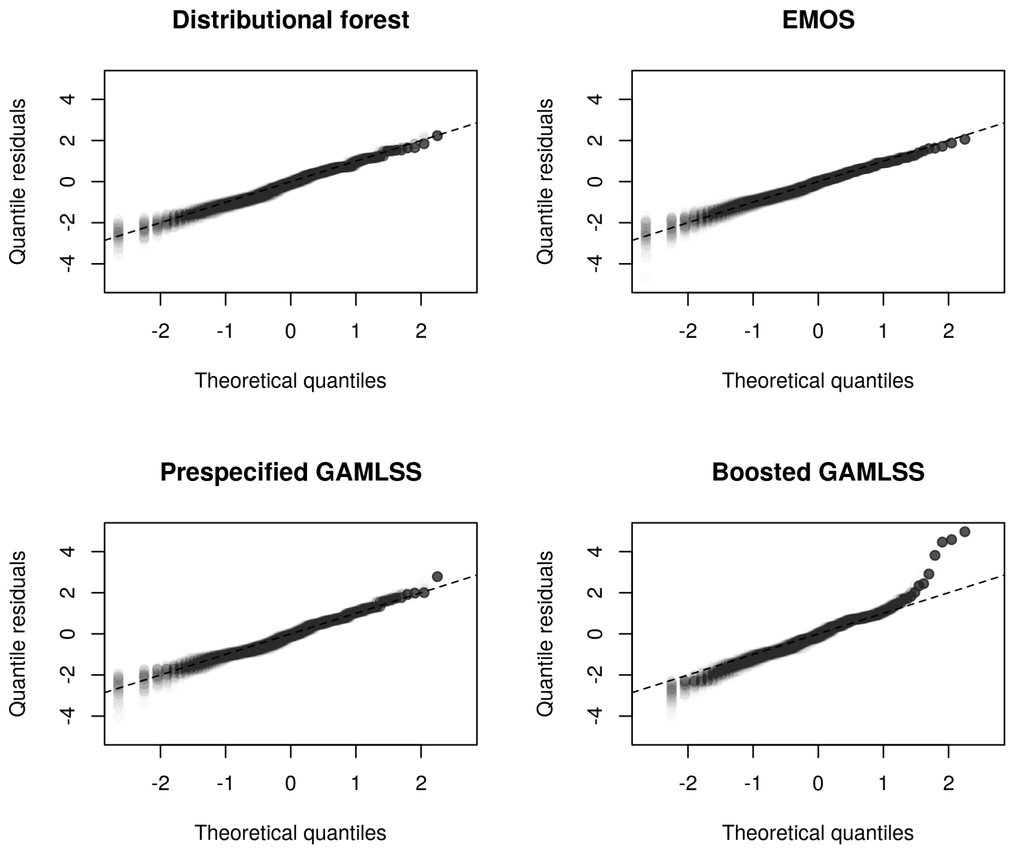


## PIT histograms

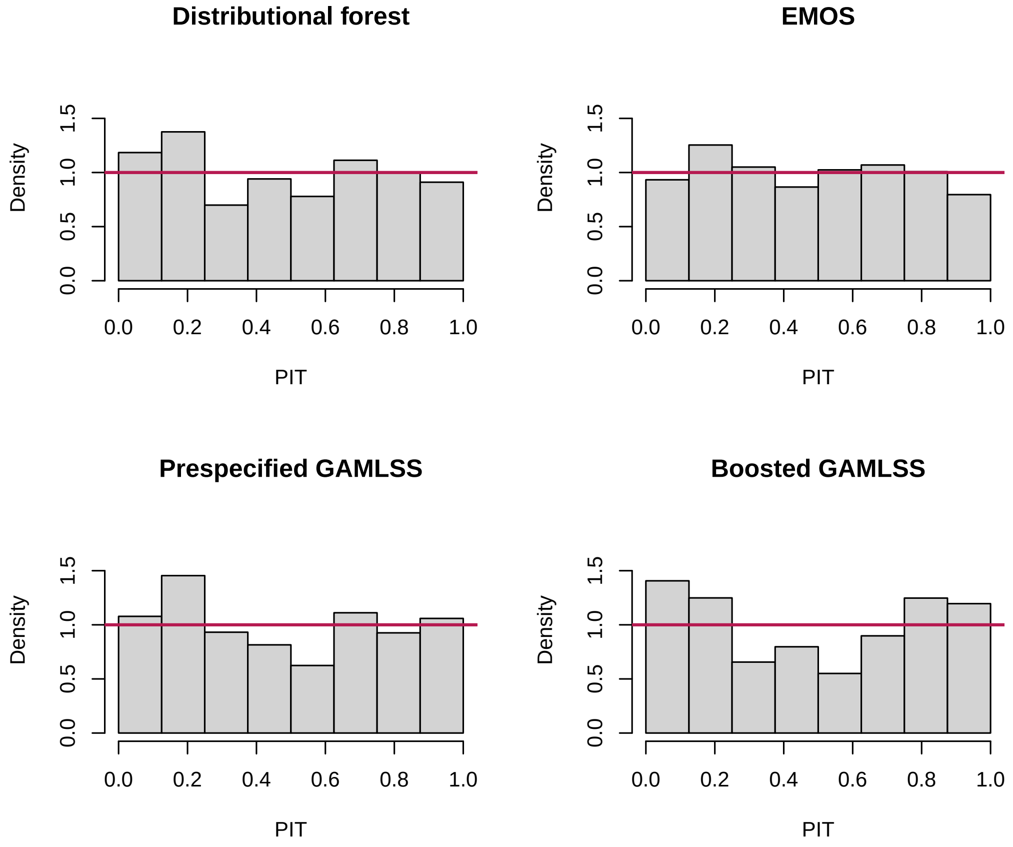

# Matrei in Osttirol

Longitude: 12.544
Latitude: 47.004
Altitude: 1040.000

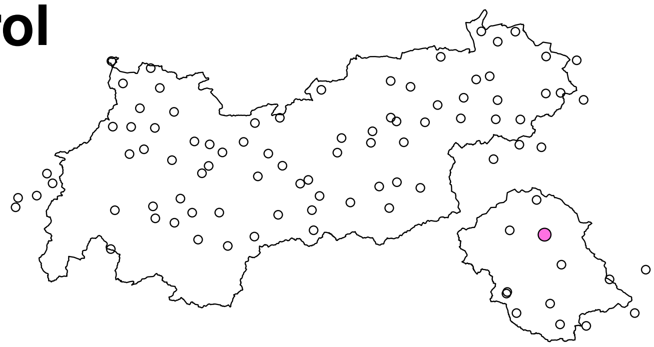

## Overview

| | Single split | | | 10 times 7-fold cross-validation | | |
|---|---|---|---|---|---|---|
| Model | CRPS | Fit time | Predict time | CRPS | Fit time | Predict time |
| Distributional forest | 0.896 | 72.474 | 0.317 | 0.724 | 81.065 | 4.351 |
| Prespecified GAMLSS | 0.844 | 79.612 | 0.255 | 0.721 | 104.928 | 0.384 |
| Boosted GAMLSS | 0.938 | 113.104 | 0.094 | 0.734 | 131.855 | 0.136 |
| *(mstop selection)* | | 1429.393 | | | 2333.012 | |
| EMOS | 0.891 | 0.083 | 0.006 | 0.787 | 0.094 | 0.006 |

## CRPS skill score (cross-validation, reference: EMOS)

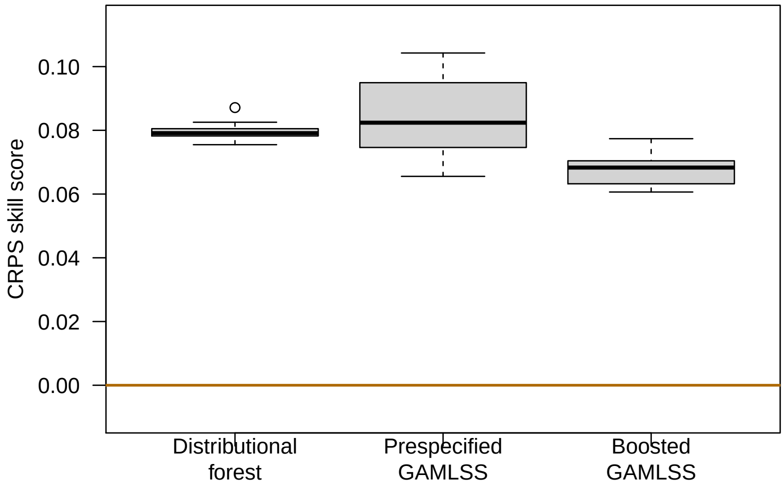


## Variable importance

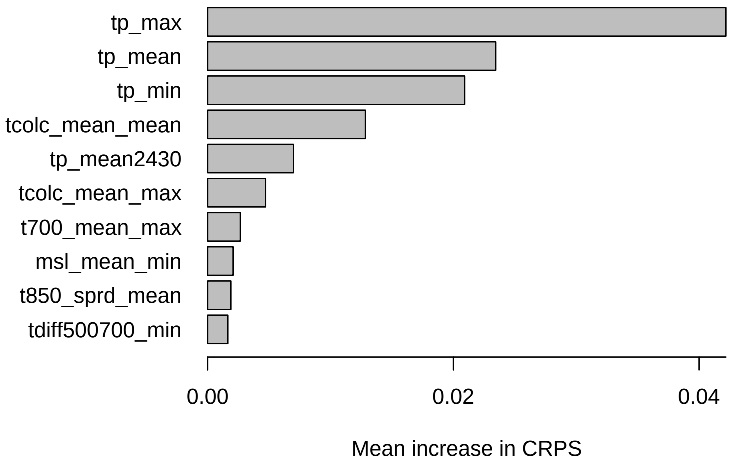

## Residual QQ plots

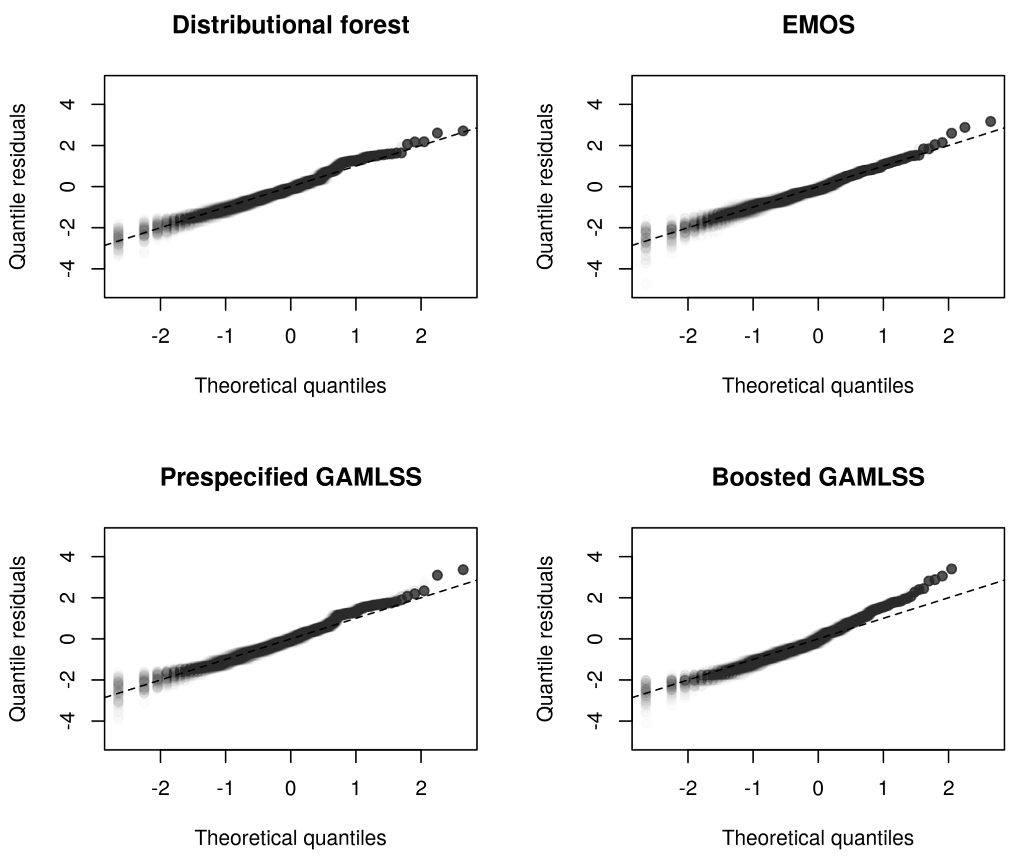


## PIT histograms

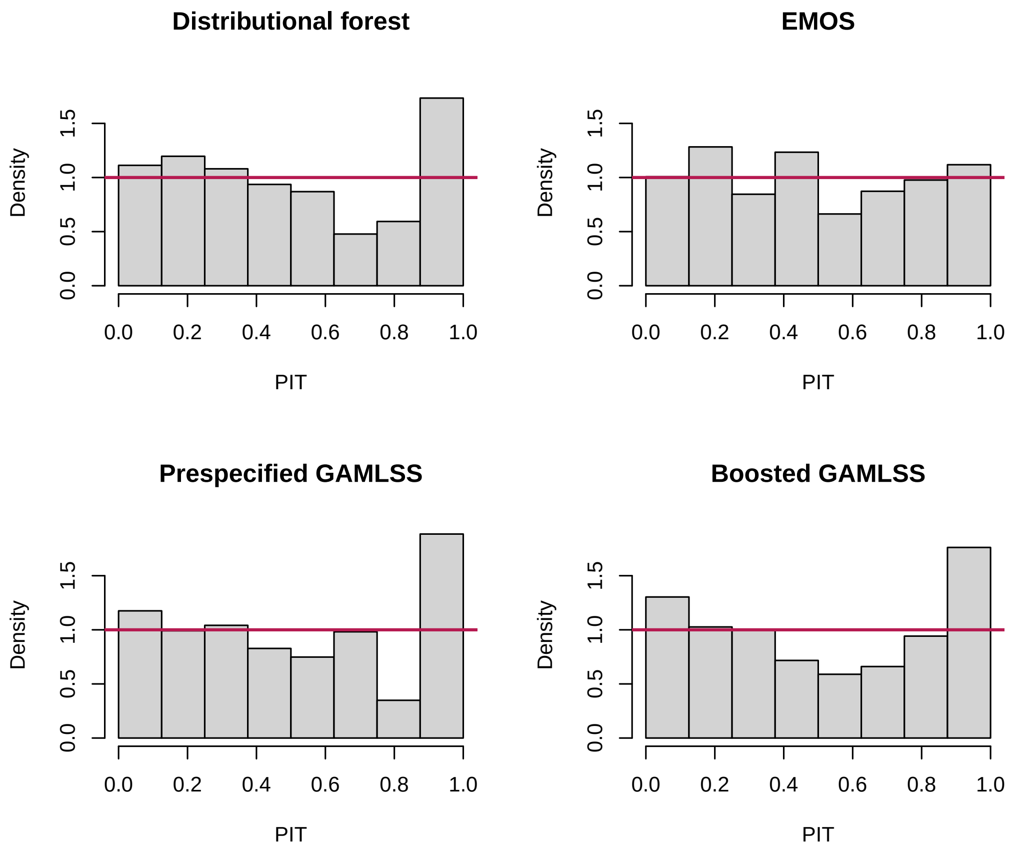

# St.Johann im Walde

Longitude: 12.626
Latitude: 46.905
Altitude: 750.000

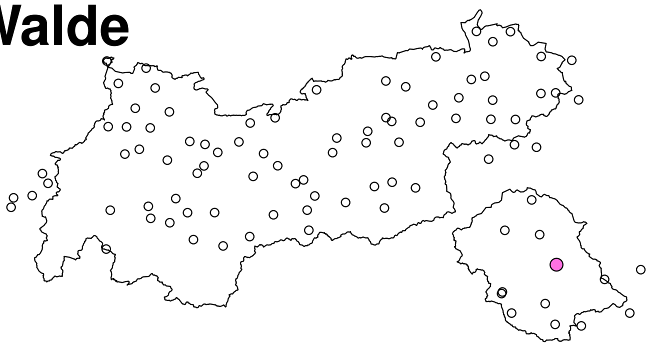

## Overview

| | Single split | | | 10 times 7-fold cross-validation | | |
|---|---|---|---|---|---|---|
| Model | CRPS | Fit time | Predict time | CRPS | Fit time | Predict time |
| Distributional forest | 0.682 | 74.754 | 0.321 | 0.710 | 87.806 | 4.696 |
| Prespecified GAMLSS | 0.616 | 46.754 | 0.253 | 0.673 | 68.119 | 0.396 |
| Boosted GAMLSS | 0.678 | 111.859 | 0.102 | 0.712 | 133.545 | 0.146 |
| *(mstop selection)* | | 1419.278 | | | 2275.568 | |
| EMOS | 0.682 | 0.084 | 0.006 | 0.767 | 0.099 | 0.005 |

## CRPS skill score (cross-validation, reference: EMOS)

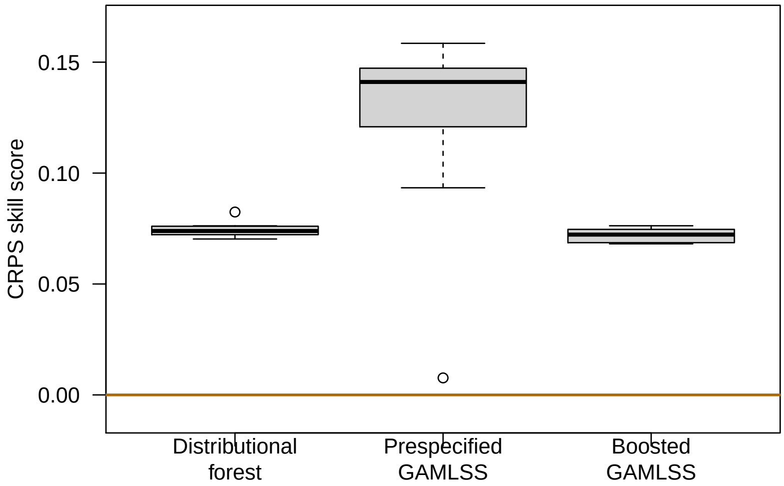


## Variable importance

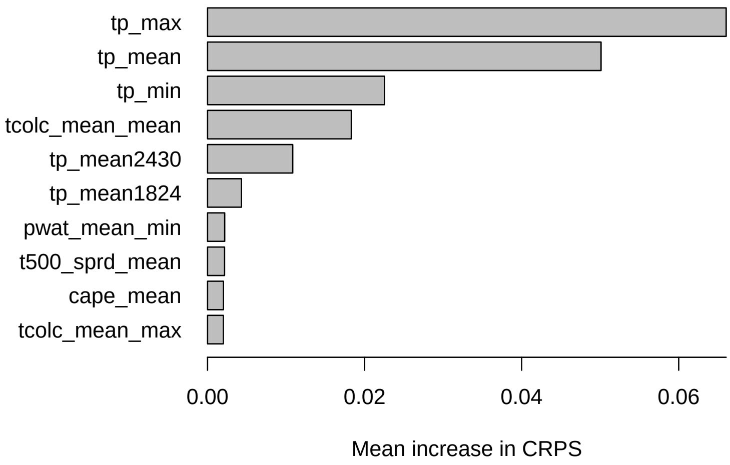

## Residual QQ plots

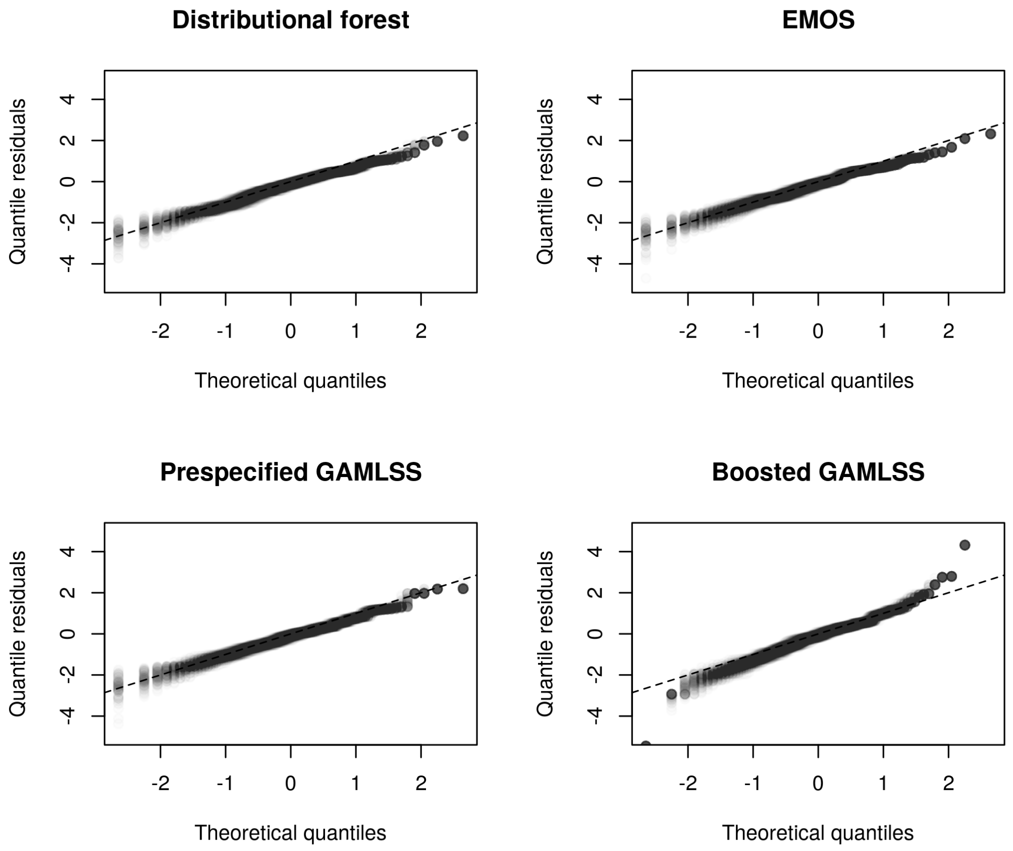


## PIT histograms

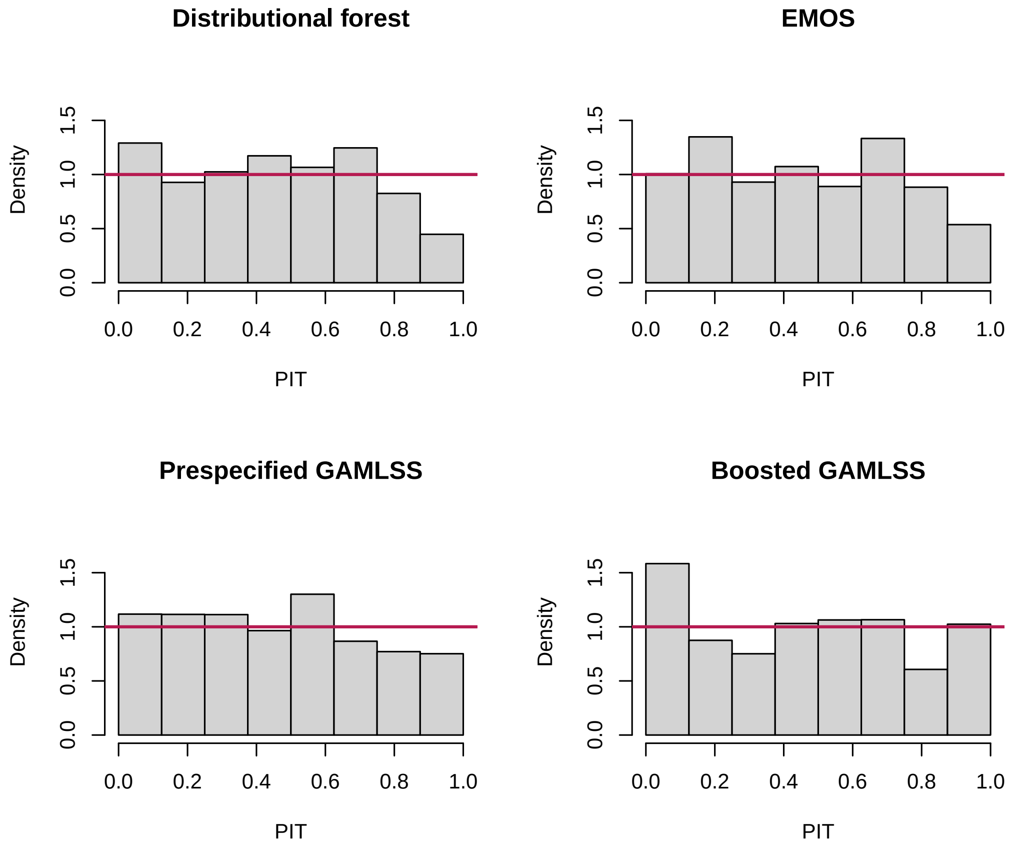

# References

Gneiting T, Raftery AE, Westveld III AH, Goldman T (2005). "Calibrated Probabilistic Forecasting Using Ensemble Model Output Statistics and Minimum CRPS Estimation." *Monthly Weather Review*, **133**(5), 1098–1118. doi:10.1175/mwr2904.1.

Hofner B, Mayr A, Schmid M (2016). "**gamboostLSS**: An R Package for Model Building and Variable Selection in the GAMLSS Framework." *Journal of Statistical Software*, **74**(1), 1–31. doi:10.18637/jss.v074.i01.

Messner JW, Mayr GJ, Zeileis A (2017). "Non-Homogeneous Boosting for Predictor Selection in Ensemble Post-Processing." *Monthly Weather Review*, **145**(1), 137–147. doi:10.1175/mwr-d-16-0088.1.

Stasinopoulos DM, Rigby RA (2007). "Generalized Additive Models for Location Scale and Shape (GAMLSS) in R." *Journal of Statistical Software*, **23**(7), 1–46. doi:10.18637/jss.v023.i07.

Stauffer R, Umlauf N, Messner JW, Mayr GJ, Zeileis A (2017). "Ensemble Post-Processing of Daily Precipitation Sums over Complex Terrain Using Censored High-Resolution Standardized Anomalies." *Monthly Weather Review*, **45**(3), 955–969. doi:10.1175/mwr-d-16-0260.1.

**Affiliation:**

Lisa Schlosser, Reto Stauffer, Achim Zeileis
Universität Innsbruck
Department of Statistics
Faculty of Economics and Statistics
Universitätsstr. 15
6020 Innsbruck, Austria
E-mail: Lisa.Schlosser@uibk.ac.at, Reto.Stauffer@uibk.ac.at, Achim.Zeileis@R-project.org
URL: https://www.uibk.ac.at/statistics/personal/schlosser-lisa/,
https://retostauffer.org/,
https://eeecon.uibk.ac.at/~zeileis/

Torsten Hothorn
Universität Zürich
Institut für Epidemiologie, Biostatistik und Prävention
Hirschengraben 84
CH-8001 Zürich, Switzerland
E-mail: Torsten.Hothorn@R-project.org
URL: http://user.math.uzh.ch/hothorn/
